# Supplementary material for: HOMFLY Polynomials of Pretzel Knots
Source: arXiv:2101.00695 ancillary file (2021-01-03)
Supplement: Supplementary file 1 [file ancillary_tables.pdf]

## Differences For Selected Knots

In Table 7, we list the differences with  $a = b = 1$  for  $r = 4$ . In particular, we list 5 first differences, and at each level one less difference, to support the conjecture that in fact the  $r^{\text{th}}$  differences seem to be constant in representation  $r$  up to a monomial factor. Further values are listed in the repository. The differences here are  $Q^n(c, r)$  rather than  $Q^{(n)}(c, r)$  with the slight difference that the monomial factors are made the same when subtracting (in particular, we divide out the first operand by precisely the factor in the remark)

**Remark 1.** The monomial factors within a difference number  $n$  seem to always increase by a factor of  $A^{2(n-1)}q^{2(n-2)(n-1)}$  as  $c$  increases by 2.

| n | c | r | difference                                                                                                                                                                                                                                                                                                                                                                                                                                                                                                                                                                                                                                                                                                                                                                                                                                                                                                                                                                                                                                                                                                                                                                                                                                                                                                                                |
|---|---|---|-------------------------------------------------------------------------------------------------------------------------------------------------------------------------------------------------------------------------------------------------------------------------------------------------------------------------------------------------------------------------------------------------------------------------------------------------------------------------------------------------------------------------------------------------------------------------------------------------------------------------------------------------------------------------------------------------------------------------------------------------------------------------------------------------------------------------------------------------------------------------------------------------------------------------------------------------------------------------------------------------------------------------------------------------------------------------------------------------------------------------------------------------------------------------------------------------------------------------------------------------------------------------------------------------------------------------------------------|
| 4 | 1 | 4 | $(A-1)A^8(A+1)q^{22}(A-q)(A+q)(Aq-1)(Aq+1)(Aq^2-1)(Aq^4-1)(Aq^5+1)(Aq^6-1)(Aq^6+1)(A^2q^6+1)(Aq^7-1)(Aq^7+1)(A^2q^8-Aq^4+1)(A^2q^8+Aq^4+1)(A^2q^{10}+1)(A^4q^{12}+1)$                                                                                                                                                                                                                                                                                                                                                                                                                                                                                                                                                                                                                                                                                                                                                                                                                                                                                                                                                                                                                                                                                                                                                                     |
| 4 | 3 | 4 | $(A-1)A^{16}(A+1)q^{46}(A-q)(A+q)(Aq-1)(Aq+1)(Aq^2-1)(Aq^4-1)(Aq^5+1)(Aq^6-1)(Aq^6+1)(A^2q^6+1)(Aq^7-1)(Aq^7+1)(A^2q^8-Aq^4+1)(A^2q^8+Aq^4+1)(A^2q^{10}+1)(A^4q^{12}+1)$                                                                                                                                                                                                                                                                                                                                                                                                                                                                                                                                                                                                                                                                                                                                                                                                                                                                                                                                                                                                                                                                                                                                                                  |
| 3 | 1 | 4 | $(A-1)A^8(A+1)q^8(A-q)(A+q)(Aq-1)(Aq+1)(Aq^4-1)(Aq^5+1)(Aq^6-1)(Aq^6+1)(A^2q^6+1)(A^10q^{54}+A^{10}q^{50}+A^{10}q^{48}+A^{10}q^{46}-A^{10}q^{44}-A^8q^{44}+2A^8q^{40}+A^8q^{38}-A^8q^{32}-A^6q^{42}+A^6q^{30}+A^6q^{28}-A^4q^{34}-A^4q^{28}-A^4q^{14}-A^4q^{12}-A^4q^{10}-A^4q^8-A^2q^{26}-A^2q^{24}-A^2q^{22}+A^2q^{20}+A^2q^{18}-A^2q^{10}-A^2q^8-q^6-q^4-q^2-1)$                                                                                                                                                                                                                                                                                                                                                                                                                                                                                                                                                                                                                                                                                                                                                                                                                                                                                                                                                                       |
| 3 | 3 | 4 | $(A-1)A^{14}(A+1)q^{20}(A-q)(A+q)(Aq-1)(Aq+1)(Aq^4-1)(Aq^5+1)(Aq^6-1)(Aq^6+1)(A^2q^6+1)(A^{14}q^{70}-A^{12}q^{66}+A^{12}q^{62}+A^{12}q^{60}+A^{12}q^{58}-A^{12}q^{56}-A^{10}q^{56}+2A^{10}q^{52}+A^{10}q^{50}-A^{10}q^{44}-A^8q^{54}+A^8q^{42}-A^6q^{44}+A^6q^{40}+A^6q^{28}-A^6q^{20}-A^4q^{38}-A^4q^{36}-A^4q^{34}+A^4q^{32}+A^4q^{30}-A^4q^{28}-A^2q^{28}+A^2q^{26}+A^2q^{24}-A^2q^{22}+A^2q^{20}-A^2q^{18}-A^2q^{10}-A^2q^8-A^2q^6-q^8-q^6-q^4-q^2-1)$                                                                                                                                                                                                                                                                                                                                                                                                                                                                                                                                                                                                                                                                                                                                                                                                                                                                                |
| 3 | 5 | 4 | $(A-1)A^{20}(A+1)q^{32}(A-q)(A+q)(Aq-1)(Aq+1)(Aq^4-1)(Aq^5+1)(Aq^6-1)(Aq^6+1)(A^2q^6+1)(A^{16}q^{82}-A^{14}q^{78}+A^{14}q^{74}+A^{14}q^{72}+A^{14}q^{70}-A^{14}q^{68}-A^{12}q^{68}+2A^{12}q^{64}+A^{12}q^{62}-A^{12}q^{56}-A^{10}q^{66}+A^{10}q^{54}+A^{10}q^{52}-A^8q^{58}-A^8q^{56}+A^8q^{52}+A^8q^{40}-A^8q^{32}-A^6q^{48}-A^6q^{46}-A^6q^{44}+A^6q^{42}-A^6q^{38}-A^6q^{36}-A^6q^{34}+A^6q^{32}-A^6q^{30}-A^4q^{46}-A^4q^{44}-A^4q^{42}+A^4q^{40}-A^4q^{38}-A^4q^{36}-A^4q^{34}-A^4q^{32}+A^4q^{30}+A^4q^{28}+2A^4q^{26}+A^4q^{24}-3A^4q^{22}-3A^4q^{20}-3A^4q^{18}+2A^4q^{14}+2A^4q^{12}+A^4q^{10}+A^2q^{36}+2A^2q^{34}-A^2q^{30}-3A^2q^{28}+3A^2q^{24}+3A^2q^{22}+3A^2q^{20}-A^2q^{18}-A^2q^{16}-A^2q^{14}-A^2q^{12}+A^2q^{10}+A^2q^8+2A^2q^6+A^2q^4+A^2q^2+q^{18}+3q^{16}+3q^{14}-q^{10}-q^8+2q^4+q^2+1)$                                                                                                                                                                                                                                                                                                                                                                                                                                                                                                                          |
| 2 | 1 | 4 | $\frac{1}{q^2}(A-1)A^8(A+1)(A-q)(A+q)(Aq^4-1)(Aq^5-1)(Aq^5+1)(A^{14}q^{68}-A^{12}q^{66}-A^{12}q^{64}+A^{12}q^{62}+A^{12}q^{60}-A^{12}q^{58}-A^{10}q^{62}-A^{10}q^{60}-2A^{10}q^{58}-A^{10}q^{56}+3A^{10}q^{52}+2A^{10}q^{50}-A^{10}q^{46}-A^{10}q^{44}+A^8q^{56}-A^8q^{52}-2A^8q^{50}-3A^8q^{48}+A^8q^{46}+2A^8q^{44}+3A^8q^{42}+A^8q^{40}-2A^8q^{38}-2A^8q^{36}-2A^8q^{34}-A^8q^{32}+A^6q^{50}-2A^6q^{44}-2A^6q^{42}-A^6q^{40}-A^6q^{38}+3A^6q^{36}+3A^6q^{34}+A^6q^{32}-A^6q^{30}-4A^6q^{28}-4A^6q^{26}-A^6q^{24}+A^6q^{22}+A^6q^{20}+A^6q^{18}+A^4q^{44}+A^4q^{42}+A^4q^{40}-2A^4q^{38}-2A^4q^{36}-A^4q^{34}-A^4q^{32}+3A^4q^{30}+A^4q^{28}+2A^4q^{26}+A^4q^{24}-3A^4q^{22}-3A^4q^{20}-3A^4q^{18}+2A^4q^{14}+2A^4q^{12}+A^4q^{10}+A^2q^{36}+2A^2q^{34}-A^2q^{30}-3A^2q^{28}+3A^2q^{24}+3A^2q^{22}+3A^2q^{20}-A^2q^{18}-A^2q^{16}-A^2q^{14}-A^2q^{12}+A^2q^{10}+A^2q^8+2A^2q^6+A^2q^4+A^2q^2+q^{28}+q^{26}+q^{24}-q^{22}+q^{18}+3q^{16}+3q^{14}-q^{10}-q^8+2q^4+q^2+1)$                                                                                                                                                                                                                                                                                                                                                                 |
| 2 | 3 | 4 | $(A-1)A^{12}(A+1)(A-q)q^2(A+q)(Aq^4-1)(Aq^5+1)(Aq^5-1)(Aq^5+1)(A^{18}q^{88}-A^{16}q^{86}-A^{16}q^{84}+A^{16}q^{82}+A^{16}q^{80}-A^{14}q^{80}+A^{16}q^{78}-2A^{14}q^{78}-A^{14}q^{76}+A^{12}q^{76}-A^{16}q^{74}+3A^{14}q^{72}-A^{12}q^{72}-2A^{14}q^{70}-2A^{12}q^{70}-3A^{12}q^{68}-A^{14}q^{66}+A^{12}q^{66}-A^{14}q^{64}+2A^{12}q^{64}-2A^{10}q^{64}+A^8q^{64}+3A^{12}q^{62}-2A^{10}q^{62}+A^8q^{62}+A^{12}q^{60}-A^{10}q^{60}+A^8q^{60}-A^{12}q^{58}-2A^8q^{58}-A^{12}q^{56}+2A^{10}q^{56}-2A^8q^{56}+A^6q^{56}-A^{12}q^{54}+2A^{10}q^{54}-A^8q^{54}+2A^6q^{54}+2A^{10}q^{52}-A^8q^{52}+A^{10}q^{50}+A^8q^{50}-A^{10}q^{48}-3A^6q^{48}+A^4q^{48}-2A^{10}q^{46}+A^8q^{46}-2A^6q^{46}+A^4q^{46}-2A^{10}q^{44}+3A^8q^{44}+A^6q^{44}+2A^4q^{44}-A^{10}q^{42}+3A^8q^{42}-A^4q^{42}-A^{10}q^{40}-2A^4q^{40}-3A^8q^{38}+A^6q^{38}-2A^4q^{38}+A^2q^{38}-4A^8q^{36}+3A^6q^{36}+A^4q^{36}+A^2q^{36}-4A^8q^{34}+3A^6q^{34}+3A^4q^{34}+A^2q^{34}+A^6q^{32}+2A^4q^{32}-2A^2q^{32}+A^8q^{30}+3A^4q^{30}-2A^2q^{30}+A^8q^{28}-5A^6q^{28}+2A^4q^{28}+q^{28}+A^8q^{26}-3A^6q^{26}+2A^2q^{26}-A^4q^{24}+5A^2q^{24}+3A^6q^{22}-3A^4q^{22}+3A^2q^{22}-2A^6q^{20}-3A^4q^{20}+A^6q^{18}-2A^4q^{18}-2A^2q^{18}+2q^{18}+A^4q^{16}-2A^2q^{16}+2q^{16}+2A^4q^{14}-A^2q^{14}+2A^4q^{12}-q^{12}+A^4q^{10}+A^2q^{10}-2q^{10}+A^2q^8-q^8+2A^2q^6+A^2q^4+2q^4+q^2+1)$ |
| 2 | 5 | 4 | $(A-1)A^{16}(A+1)(A-q)q^6(A+q)(Aq^4-1)(Aq^5+1)(Aq^5-1)(Aq^5+1)(A^{22}q^{108}-A^{20}q^{106}-A^{20}q^{104}+A^{20}q^{102}+A^{20}q^{100}-A^{18}q^{100}+A^{20}q^{98}-2A^{18}q^{98}-A^{18}q^{96}+A^{16}q^{96}-A^{20}q^{94}+3A^{18}q^{92}-A^{16}q^{92}+2A^{18}q^{90}-2A^{16}q^{90}+A^{14}q^{90}-3A^{16}q^{88}-A^{18}q^{86}-A^{16}q^{84}+2A^{16}q^{84}-2A^{14}q^{84}+A^{12}q^{84}+3A^{16}q^{82}-2A^{14}q^{82}+A^{12}q^{82}+A^{16}q^{80}-A^{14}q^{80}+A^{12}q^{80}-A^{16}q^{$                                                                                                                                                                                                                                                                                                                                                                                                                                                                                                                                                                                                                                                                                                                                                                                                                                                                      |

[illegible]

| n | c | r | difference                                                                                                                                                                                                                                                                                                                                                                                                                                                                                                                                                                                                                                                                                                                                                                                                                                                                                                                                                                                                                                                                                                                                                                                                                                                                                                                                                                                                                                                                                                                                                                                                                                                                                                                                                                                                                                                                                                                                                                                                                                                                                                                                                                                                                                                                                                                                                                                                                                                                                                                                                                                                                                                                                                                                                                                                                                                                                                                                                                                                                                                                                                                                                                                                                                                                                                                                                                                                                                                                                                                                                                                                                                       |
|---|---|---|--------------------------------------------------------------------------------------------------------------------------------------------------------------------------------------------------------------------------------------------------------------------------------------------------------------------------------------------------------------------------------------------------------------------------------------------------------------------------------------------------------------------------------------------------------------------------------------------------------------------------------------------------------------------------------------------------------------------------------------------------------------------------------------------------------------------------------------------------------------------------------------------------------------------------------------------------------------------------------------------------------------------------------------------------------------------------------------------------------------------------------------------------------------------------------------------------------------------------------------------------------------------------------------------------------------------------------------------------------------------------------------------------------------------------------------------------------------------------------------------------------------------------------------------------------------------------------------------------------------------------------------------------------------------------------------------------------------------------------------------------------------------------------------------------------------------------------------------------------------------------------------------------------------------------------------------------------------------------------------------------------------------------------------------------------------------------------------------------------------------------------------------------------------------------------------------------------------------------------------------------------------------------------------------------------------------------------------------------------------------------------------------------------------------------------------------------------------------------------------------------------------------------------------------------------------------------------------------------------------------------------------------------------------------------------------------------------------------------------------------------------------------------------------------------------------------------------------------------------------------------------------------------------------------------------------------------------------------------------------------------------------------------------------------------------------------------------------------------------------------------------------------------------------------------------------------------------------------------------------------------------------------------------------------------------------------------------------------------------------------------------------------------------------------------------------------------------------------------------------------------------------------------------------------------------------------------------------------------------------------------------------------------|
| 1 | 5 | 4 | $\frac{A^{14}}{q^8}(A-q)(Aq^4-1)(Aq^4+1)(A^{30}q^{132}-A^{28}q^{130}+A^{26}q^{128}-A^{28}q^{126}-A^{24}q^{124}-2A^{26}q^{124}+A^{24}q^{124}-2A^{26}q^{122}+2A^{24}q^{122}+A^{24}q^{120}-A^{22}q^{120}-A^{28}q^{118}+2A^{26}q^{116}-4A^{24}q^{116}+2A^{22}q^{116}+A^{26}q^{114}-A^{20}q^{114}-A^{26}q^{112}+A^{22}q^{112}-A^{26}q^{110}+3A^{24}q^{110}-3A^{22}q^{110}+A^{20}q^{110}-3A^{24}q^{108}-5A^{22}q^{108}+3A^{20}q^{108}-A^{18}q^{108}-2A^{22}q^{106}+3A^{20}q^{106}-A^{18}q^{106}-A^{24}q^{104}+A^{22}q^{104}-A^{24}q^{102}+4A^{22}q^{102}-4A^{20}q^{102}+A^{18}q^{102}+2A^{22}q^{100}-5A^{20}q^{100}+4A^{18}q^{100}-A^{16}q^{100}-A^{20}q^{98}+2A^{18}q^{98}-A^{16}q^{98}-A^{22}q^{96}+2A^{20}q^{96}-A^{18}q^{96}-A^{22}q^{94}+4A^{20}q^{94}-5A^{18}q^{94}+2A^{16}q^{94}+2A^{20}q^{92}-5A^{18}q^{92}+4A^{16}q^{92}-A^{14}q^{92}-A^{18}q^{90}-A^{14}q^{90}-A^{20}q^{88}+2A^{18}q^{88}-A^{16}q^{88}-A^{20}q^{86}+4A^{18}q^{86}-5A^{16}q^{86}+2A^{14}q^{86}+2A^{18}q^{84}-A^{16}q^{84}-A^{12}q^{84}-A^{16}q^{82}+2A^{14}q^{82}-A^{12}q^{82}-A^{18}q^{80}+2A^{16}q^{80}-A^{14}q^{80}-A^{20}q^{78}+4A^{16}q^{78}-5A^{14}q^{78}+2A^{12}q^{78}-A^{20}q^{76}+A^{16}q^{76}-5A^{14}q^{76}+4A^{12}q^{76}-A^{10}q^{76}-A^{20}q^{74}+2A^{18}q^{74}-A^{16}q^{74}-A^{14}q^{74}+2A^{12}q^{74}-A^{10}q^{74}-A^{20}q^{72}+2A^{14}q^{72}-A^{12}q^{72}-2A^{18}q^{70}+3A^{16}q^{70}+2A^{14}q^{70}-5A^{12}q^{70}+2A^{10}q^{70}-2A^{18}q^{68}+4A^{16}q^{68}-5A^{12}q^{68}+4A^{10}q^{68}-A^{8}q^{68}-2A^{18}q^{66}+A^{16}q^{66}+3A^{14}q^{66}-3A^{12}q^{66}+2A^{10}q^{66}-A^{8}q^{66}+4A^{16}q^{64}-2A^{12}q^{64}+2A^{18}q^{62}-7A^{16}q^{62}+8A^{14}q^{62}-5A^{10}q^{62}+2A^{8}q^{62}+A^{18}q^{60}-4A^{16}q^{60}+4A^{12}q^{60}-7A^{10}q^{60}+6A^{8}q^{60}-A^{6}q^{60}+5A^{14}q^{64}-2A^{12}q^{64}+10A^{12}q^{58}-7A^{10}q^{58}+3A^{8}q^{58}-A^{6}q^{58}+4A^{16}q^{56}-10A^{14}q^{56}+9A^{12}q^{56}-3A^{10}q^{56}+3A^{16}q^{54}-9A^{14}q^{54}+5A^{12}q^{54}+7A^{10}q^{54}-8A^{8}q^{54}+2A^{6}q^{54}+A^{16}q^{52}+A^{14}q^{52}-8A^{12}q^{52}+13A^{10}q^{52}-11A^{8}q^{52}+5A^{6}q^{52}-A^{4}q^{52}+5A^{14}q^{50}-15A^{12}q^{50}+16A^{10}q^{50}-8A^{8}q^{50}+3A^{6}q^{50}-A^{4}q^{50}-A^{6}q^{50}-A^{16}q^{48}+6A^{14}q^{48}-11A^{12}q^{48}+5A^{10}q^{48}+4A^{8}q^{48}-3A^{6}q^{48}+3A^{14}q^{46}-4A^{12}q^{46}-7A^{10}q^{46}+17A^{8}q^{46}-12A^{6}q^{46}+3A^{4}q^{46}-A^{14}q^{44}+7A^{12}q^{44}-16A^{10}q^{44}+18A^{8}q^{44}-12A^{6}q^{44}+5A^{4}q^{44}-A^{2}q^{44}-A^{14}q^{42}+7A^{12}q^{42}-14A^{10}q^{42}+10A^{8}q^{42}-A^{6}q^{42}-A^{2}q^{42}-A^{14}q^{40}+3A^{10}q^{40}-9A^{8}q^{40}+14A^{6}q^{40}-7A^{4}q^{40}+A^{2}q^{40}+A^{12}q^{38}+5A^{10}q^{38}-18A^{8}q^{38}+21A^{6}q^{38}-12A^{4}q^{38}+3A^{2}q^{38}-2A^{12}q^{36}+10A^{10}q^{36}-16A^{8}q^{36}+11A^{6}q^{36}-4A^{4}q^{36}+2A^{2}q^{36}-q^{36}-A^{12}q^{34}+7A^{10}q^{34}-6A^{8}q^{34}-7A^{6}q^{34}-A^{12}q^{32}+3A^{10}q^{32}+7A^{8}q^{32}-21A^{6}q^{32}+18A^{4}q^{32}-7A^{2}q^{32}+q^{32}+9A^{8}q^{30}-18A^{6}q^{30}+12A^{4}q^{30}-3A^{2}q^{30}-2A^{10}q^{28}+9A^{8}q^{28}-5A^{6}q^{28}-7A^{4}q^{28}+6A^{2}q^{28}-q^{28}-A^{10}q^{26}+3A^{8}q^{26}+7A^{6}q^{26}-18A^{4}q^{26}+12A^{2}q^{26}-3q^{26}-A^{10}q^{24}-A^{8}q^{24}+12A^{6}q^{24}-15A^{4}q^{24}+6A^{2}q^{24}-q^{24}-2A^{8}q^{22}+7A^{6}q^{22}-2A^{4}q^{22}-5A^{2}q^{22}+2q^{22}-3A^{8}q^{20}+2A^{6}q^{20}+10A^{4}q^{20}-12A^{2}q^{20}+3q^{20}-A^{8}q^{18}-3A^{6}q^{18}+10A^{4}q^{18}-8A^{2}q^{18}+2q^{18}-A^{8}q^{16}+5A^{4}q^{16}+2A^{2}q^{16}-3q^{16}-2A^{6}q^{14}-A^{4}q^{14}+7A^{2}q^{14}-4q^{14}-A^{6}q^{12}-3A^{4}q^{12}+6A^{2}q^{12}-2q^{12}-2A^{4}q^{10}+A^{2}q^{10}+q^{10}-A^{4}q^8-2A^2q^8+3q^8-2A^2q^6+q^6-A^2q^4-q^2-1)$ |
| 1 | 7 | 4 | $\frac{A^{14}}{q^8}(A-q)(Aq^4-1)(Aq^4+1)(A^{30}q^{132}-A^{28}q^{130}+A^{26}q^{128}-A^{28}q^{126}-A^{24}q^{124}-2A^{26}q^{124}+A^{24}q^{124}-2A^{26}q^{122}+2A^{24}q^{122}+A^{24}q^{120}-A^{22}q^{120}-A^{28}q^{118}+2A^{26}q^{116}-4A^{24}q^{116}+2A^{22}q^{116}+A^{26}q^{114}-A^{20}q^{114}-A^{26}q^{112}+A^{22}q^{112}-A^{26}q^{110}+3A^{24}q^{110}-3A^{22}q^{110}+A^{20}q^{110}-3A^{24}q^{108}-5A^{22}q^{108}+3A^{20}q^{108}-A^{18}q^{108}-2A^{22}q^{106}+3A^{20}q^{106}-A^{18}q^{106}-A^{24}q^{104}+A^{22}q^{104}-A^{24}q^{102}+4A^{22}q^{102}-4A^{20}q^{102}+A^{18}q^{102}+2A^{22}q^{100}-5A^{20}q^{100}+4A^{18}q^{100}-A^{16}q^{100}-A^{20}q^{98}+2A^{18}q^{98}-A^{16}q^{98}-A^{22}q^{96}+2A^{20}q^{96}-A^{18}q^{96}-A^{22}q^{94}+4A^{20}q^{94}-5A^{18}q^{94}+2A^{16}q^{94}+2A^{20}q^{92}-5A^{18}q^{92}+4A^{16}q^{92}-A^{14}q^{92}-A^{18}q^{90}-A^{14}q^{90}-A^{20}q^{88}+2A^{18}q^{88}-A^{16}q^{88}-A^{20}q^{86}+4A^{18}q^{86}-5A^{16}q^{86}+2A^{14}q^{86}+2A^{18}q^{84}-A^{16}q^{84}-A^{12}q^{84}-A^{16}q^{82}+2A^{14}q^{82}-A^{12}q^{82}-A^{18}q^{80}+2A^{16}q^{80}-A^{14}q^{80}-A^{20}q^{78}+4A^{16}q^{78}-5A^{14}q^{78}+2A^{12}q^{78}-A^{20}q^{76}+A^{16}q^{76}-5A^{14}q^{76}+4A^{12}q^{76}-A^{10}q^{76}-A^{20}q^{74}+2A^{18}q^{74}-A^{16}q^{74}-A^{14}q^{74}+2A^{12}q^{74}-A^{10}q^{74}-A^{20}q^{72}+2A^{14}q^{72}-A^{12}q^{72}-2A^{18}q^{70}+3A^{16}q^{70}+2A^{14}q^{70}-5A^{12}q^{70}+2A^{10}q^{70}-2A^{18}q^{68}+4A^{16}q^{68}-5A^{12}q^{68}+4A^{10}q^{68}-A^{8}q^{68}-2A^{18}q^{6$                                                                                                                                                                                                                                                                                                                                                                                                                                                                                                                                                                                                                                                                                                                                                                                                                                                                                                                                                                                                                                                                                                                                                                                                                                                                                                                                                                                                                                                                                                                                                                                                                                                                                                                                                                                                                                                                                                                                                                                                                                                                                                                                               |

| n | c | r | difference                                                                                                                                                                                                                                                                                                                                                                                                                                                                                                                                                                                                                                                                                                                                                                                                                                                                                                                                                                                                                                                                                                                                                                                                                                                                                                                                                                                                                                                                                                                                                                                                                                                                                                                                                                                                                                                                                                                                                                                                                                                                                                                                                                                                                                                                                                                                                                                                                                                                                                                                                                                                                                                                                                                                                                                                                                                                                                                                                                                                                                                                                                                                                                                                                                                                                                                                                                                                                                                                                                                                                                                                                                                                                                                                                                                                                                                                                                                                                                                                                                                                                                                                                                                                                                                                                                                                                                                                                                                                                                                                                                                                                                                                                                                                                                                                                                                                                                               |
|---|---|---|--------------------------------------------------------------------------------------------------------------------------------------------------------------------------------------------------------------------------------------------------------------------------------------------------------------------------------------------------------------------------------------------------------------------------------------------------------------------------------------------------------------------------------------------------------------------------------------------------------------------------------------------------------------------------------------------------------------------------------------------------------------------------------------------------------------------------------------------------------------------------------------------------------------------------------------------------------------------------------------------------------------------------------------------------------------------------------------------------------------------------------------------------------------------------------------------------------------------------------------------------------------------------------------------------------------------------------------------------------------------------------------------------------------------------------------------------------------------------------------------------------------------------------------------------------------------------------------------------------------------------------------------------------------------------------------------------------------------------------------------------------------------------------------------------------------------------------------------------------------------------------------------------------------------------------------------------------------------------------------------------------------------------------------------------------------------------------------------------------------------------------------------------------------------------------------------------------------------------------------------------------------------------------------------------------------------------------------------------------------------------------------------------------------------------------------------------------------------------------------------------------------------------------------------------------------------------------------------------------------------------------------------------------------------------------------------------------------------------------------------------------------------------------------------------------------------------------------------------------------------------------------------------------------------------------------------------------------------------------------------------------------------------------------------------------------------------------------------------------------------------------------------------------------------------------------------------------------------------------------------------------------------------------------------------------------------------------------------------------------------------------------------------------------------------------------------------------------------------------------------------------------------------------------------------------------------------------------------------------------------------------------------------------------------------------------------------------------------------------------------------------------------------------------------------------------------------------------------------------------------------------------------------------------------------------------------------------------------------------------------------------------------------------------------------------------------------------------------------------------------------------------------------------------------------------------------------------------------------------------------------------------------------------------------------------------------------------------------------------------------------------------------------------------------------------------------------------------------------------------------------------------------------------------------------------------------------------------------------------------------------------------------------------------------------------------------------------------------------------------------------------------------------------------------------------------------------------------------------------------------------------------------------------------------------|
| 1 | 9 | 4 | $\frac{A^{15}}{q^8}(A-q)(A+q)(Aq^4-1)(Aq^4+1)(A^{36}q^{156}-A^{34}q^{156}-A^{34}q^{154}+A^{32}q^{154}-A^{34}q^{152}+A^{32}q^{152}+A^{34}q^{150}-A^{30}q^{150}+A^{34}q^{148}-2A^{32}q^{148}+A^{30}q^{148}-2A^{32}q^{146}+2A^{30}q^{146}+A^{30}q^{144}-A^{28}q^{144}-A^{34}q^{142}+2A^{32}q^{142}-A^{30}q^{142}+2A^{32}q^{140}-A^{30}q^{140}+2A^{28}q^{140}+A^{32}q^{138}-2A^{30}q^{138}+2A^{28}q^{138}-A^{26}q^{138}-A^{32}q^{136}+A^{28}q^{136}+3A^{30}q^{134}-3A^{28}q^{134}+A^{26}q^{134}+3A^{30}q^{132}-5A^{28}q^{132}+3A^{26}q^{132}-A^{24}q^{132}-2A^{28}q^{130}+3A^{26}q^{130}-A^{24}q^{130}-A^{30}q^{128}+A^{28}q^{128}-A^{30}q^{126}+4A^{28}q^{126}-4A^{26}q^{126}+A^{24}q^{126}+2A^{28}q^{124}-5A^{26}q^{124}+4A^{24}q^{124}-A^{22}q^{124}-A^{26}q^{122}+2A^{24}q^{122}-A^{22}q^{122}-A^{28}q^{120}+2A^{26}q^{120}-A^{24}q^{120}-A^{28}q^{118}+4A^{26}q^{118}-5A^{24}q^{118}+2A^{22}q^{118}+2A^{26}q^{116}-5A^{24}q^{116}+4A^{22}q^{116}-A^{20}q^{116}-A^{24}q^{114}+2A^{22}q^{114}-A^{20}q^{114}-A^{26}q^{112}+2A^{24}q^{112}-A^{22}q^{112}-A^{26}q^{110}+4A^{24}q^{110}-5A^{22}q^{110}+2A^{20}q^{110}+2A^{24}q^{108}-5A^{22}q^{108}+4A^{20}q^{108}-A^{18}q^{108}-A^{22}q^{106}+2A^{20}q^{106}-A^{18}q^{106}-A^{24}q^{104}+2A^{22}q^{104}-A^{20}q^{104}-A^{24}q^{102}+4A^{22}q^{102}-5A^{20}q^{102}+2A^{18}q^{102}+2A^{22}q^{100}-5A^{20}q^{100}+4A^{18}q^{100}-A^{16}q^{100}-A^{20}q^{98}+2A^{18}q^{98}-A^{16}q^{98}-A^{22}q^{96}+2A^{20}q^{96}-A^{18}q^{96}-A^{22}q^{94}+4A^{20}q^{94}-5A^{18}q^{94}+2A^{16}q^{94}+2A^{20}q^{92}-5A^{18}q^{92}+4A^{16}q^{92}-A^{14}q^{92}-A^{24}q^{90}+A^{22}q^{90}-A^{18}q^{90}+2A^{16}q^{90}-A^{14}q^{90}-A^{24}q^{88}+2A^{22}q^{88}-2A^{20}q^{88}-A^{16}q^{88}-A^{24}q^{86}+2A^{20}q^{86}-4A^{18}q^{86}-5A^{16}q^{86}+2A^{14}q^{86}-A^{24}q^{84}+A^{20}q^{84}+2A^{18}q^{84}-5A^{16}q^{84}+4A^{14}q^{84}-A^{12}q^{84}-2A^{22}q^{82}+4A^{20}q^{82}-2A^{18}q^{82}-A^{16}q^{82}+2A^{14}q^{82}-A^{12}q^{82}-2A^{22}q^{80}+4A^{20}q^{80}-3A^{18}q^{80}+2A^{16}q^{80}-A^{14}q^{80}-2A^{22}q^{78}+A^{20}q^{78}+2A^{16}q^{78}-5A^{14}q^{78}+2A^{12}q^{78}+A^{22}q^{76}-4A^{20}q^{76}+6A^{18}q^{76}-2A^{16}q^{76}-4A^{14}q^{76}+4A^{12}q^{76}-A^{10}q^{76}+2A^{22}q^{74}-7A^{20}q^{74}+9A^{18}q^{74}-4A^{16}q^{74}-A^{14}q^{74}+2A^{12}q^{74}-A^{10}q^{74}+A^{22}q^{72}-4A^{20}q^{72}+3A^{18}q^{72}+A^{16}q^{72}-A^{12}q^{72}+A^{22}q^{70}-6A^{18}q^{70}+9A^{16}q^{70}-2A^{14}q^{70}-4A^{12}q^{70}+2A^{10}q^{70}+4A^{20}q^{68}-10A^{18}q^{68}+10A^{16}q^{68}-3A^{14}q^{68}-4A^{12}q^{68}+4A^{10}q^{68}-A^{8}q^{68}+3A^{20}q^{66}-9A^{18}q^{66}+6A^{16}q^{66}+3A^{14}q^{66}-4A^{12}q^{66}+2A^{10}q^{66}-A^{8}q^{66}+A^{20}q^{64}+A^{18}q^{64}+10A^{14}q^{64}-4A^{12}q^{64}+5A^{18}q^{62}-15A^{16}q^{62}+15A^{14}q^{62}-3A^{12}q^{62}-4A^{10}q^{62}+2A^{8}q^{62}-A^{20}q^{60}+6A^{18}q^{60}-11A^{16}q^{60}+6A^{14}q^{60}+4A^{12}q^{60}-10A^{10}q^{60}+4A^{8}q^{60}-A^{6}q^{60}+3A^{18}q^{58}-4A^{16}q^{58}-6A^{14}q^{58}+13A^{12}q^{58}-8A^{10}q^{58}+3A^{8}q^{58}-A^{6}q^{58}-A^{18}q^{56}+7A^{16}q^{56}-16A^{14}q^{56}+15A^{12}q^{56}-5A^{10}q^{56}-A^{18}q^{54}+7A^{16}q^{54}-15A^{14}q^{54}+10A^{12}q^{54}+4A^{10}q^{54}-7A^{8}q^{54}+2A^{6}q^{54}-A^{18}q^{52}+5A^{16}q^{52}-4A^{14}q^{52}-7A^{12}q^{52}+14A^{10}q^{52}-11A^{8}q^{52}+5A^{6}q^{52}-A^{4}q^{52}+A^{16}q^{50}+3A^{14}q^{50}-15A^{12}q^{50}+18A^{10}q^{50}-9A^{8}q^{50}+3A^{6}q^{50}-A^{4}q^{50}-2A^{16}q^{48}+9A^{14}q^{48}-16A^{12}q^{48}+10A^{10}q^{48}+2A^{8}q^{48}-3A^{6}q^{48}-A^{16}q^{46}+6A^{14}q^{46}-7A^{12}q^{46}-4A^{10}q^{46}+14A^{8}q^{46}-11A^{6}q^{46}+3A^{4}q^{46}-A^{16}q^{44}+4A^{12}q^{44}-17A^{10}q^{44}+19A^{8}q^{44}-12A^{6}q^{44}+5A^{4}q^{44}-A^{2}q^{44}+7A^{12}q^{42}-17A^{10}q^{42}+12A^{8}q^{42}-A^{6}q^{42}-2A^{14}q^{40}+9A^{12}q^{40}-9A^{10}q^{40}-5A^{8}q^{40}+13A^{6}q^{40}-7A^{4}q^{40}+A^{2}q^{40}-A^{14}q^{38}+5A^{12}q^{38}+A^{10}q^{38}-17A^{8}q^{38}+21A^{6}q^{38}-12A^{4}q^{38}+3A^{2}q^{38}-A^{14}q^{36}+2A^{12}q^{36}+9A^{10}q^{36}-20A^{8}q^{36}+13A^{6}q^{36}-4A^{4}q^{36}+2A^{2}q^{36}-3A^0q^{36}+8A^{10}q^{34}-10A^{8}q^{34}-5A^{6}q^{34}+11A^{4}q^{34}-4A^{2}q^{34}-2A^{12}q^{32}+7A^{10}q^{32}+2A^{8}q^{32}-19A^{6}q^{32}+18A^{4}q^{32}-7A^{2}q^{32}+q^{32}-A^{12}q^{30}+2A^{10}q^{30}+9A^{8}q^{30}-19A^{6}q^{30}+12A^{4}q^{30}-3A^{2}q^{30}-A^{10}q^{28}+11A^{8}q^{28}-7A^{6}q^{28}-7A^{4}q^{28}+6A^{2}q^{28}-q^{28}-2A^{10}q^{26}+5A^{8}q^{26}+6A^{6}q^{26}-18A^{4}q^{26}+12A^2q^{26}-3q^{26}-3A^{10}q^{24}+A^8q^{24}+12A^6q^{24}-15A^4q^{24}+6A^2q^{24}-q^{24}-A^{10}q^{22}+3A^8q^{22}+9A^6q^{22}-2A^4q^{22}-5A^2q^{22}+2q^{22}-A^{10}q^{20}-3A^8q^{20}+3A^6q^{20}+10A^4q^{20}-12A^2q^{20}+3q^{20}-2A^8q^{18}-2A^6q^{18}+10A^4q^{18}-8A^2q^{18}+2q^{18}-A^{16}q^{16}+5A^4q^{16}+2A^2q^{16}-3q^{16}-2A^6q^{14}-A^4q^{14}+7A^2q^{14}-4q^{14}-A^6q^{12}-3A^4q^{12}+6A^2q^{12}-2q^{12}-2A^4q^{10}+A^2q^{10}+q^{10}-A^4q^8-2A^2q^8+3q^8-2A^2q^6+q^6-A^2q^4-q^2-1)$ |
| 0 | 1 | 4 | $\frac{A^8}{q^8}(A^8q^{44}-A^6q^{46}-A^6q^{44}-A^6q^{42}-A^6q^{40}-A^6q^{36}-A^6q^{34}-A^6q^{32}-A^6q^{30}+A^4q^{46}+A^4q^{44}+2A^4q^{42}+A^4q^{40}+2A^4q^{38}+2A^4q^{36}+3A^4q^{34}+3A^4q^{32}+2A^4q^{30}+A^4q^{28}+A^4q^{26}+A^4q^{24}+2A^4q^{22}+A^4q^{20}+A^4q^{18}-A^2q^{44}-A^2q^{42}-A^2q^{40}-2A^2q^{38}-2A^2q^{36}-3A^2q^{34}-3A^2q^{32}-2A^2q^{30}-2A^2q^{28}-2A^2q^{26}-3A^2q^{24}-3A^2q^{22}-2A^2q^{20}-A^2q^{18}-A^2q^{16}-A^2q^{14}-A^2q^{12}-A^2q^{10}-A^2q^8+q^{36}+q^{32}+q^{28}+q^{26}+2q^{24}+q^{22}+q^{20}+q^{16}+q^{14}+q^{12}+q^{10}+1)$                                                                                                                                                                                                                                                                                                                                                                                                                                                                                                                                                                                                                                                                                                                                                                                                                                                                                                                                                                                                                                                                                                                                                                                                                                                                                                                                                                                                                                                                                                                                                                                                                                                                                                                                                                                                                                                                                                                                                                                                                                                                                                                                                                                                                                                                                                                                                                                                                                                                                                                                                                                                                                                                                                                                                                                                                                                                                                                                                                                                                                                                                                                                                                                                                                                                                                                                                                                                                                                                                                                                                                                                                                                                                                                                                                                                                                                                                                                                                                                                                                                                                                                                                                                                                                                                                                                                                           |
| 0 | 3 | 4 | $\frac{A^8}{q^8}(-A^{14}q^{70}+A^{12}q^{70}+A^{16}q^{68}-A^{14}q^{68}+A^{12}q^{68}-A^{10}q^{68}-A^{14}q^{66}+2A^{12}q^{66}-A^{10}q^{66}-A^{14}q^{64}+A^8q^{64}+A^{14}q^{62}-A^8q^{62}-A^{12}q^{60}+2A^{10}q^{60}-A^8q^{60}-A^{12}q^{58}+A^6q^{58}+A^6q^{56}-A^{10}q^{56}-A^{10}q^{54}+A^{12}q^{54}-2A^{10}q^{54}+3A^8q^{54}-A^6q^{54}+A^{12}q^{52}-2A^{10}q^{52}+A^4q^{52}+3A^{10}q^{50}-2A^8q^{50}-A^4q^{50}-2A^{12}q^{48}+3A^{10}q^{48}-4A^8q^{48}+4A^6q^{48}-A^4q^{48}-A^{12}q^{46}+4A^{10}q^{46}-4A^8q^{46}+A^2q^{46}-A^{12}q^{44}+A^{10}q^{44}+3A^8q^{44}-3A^6q^{44}+A^4q^{44}-A^2q^{44}-2A^{10}q^{42}+4A^8q^{42}-5A^6q^{42}+4A^4q^{42}-A^{10}q^{40}+4A^8q^{40}-4A^6q^{40}-A^4q^{40}+A^{10}q^{38}-A^8q^{38}+6A^6q^{38}-4A^4q^{38}+A^2q^{38}-A^{10}q^{36}-6A^8q^{36}+6A^6q^{36}-5A^4q^{36}+3A^2q^{36}-A^2q^{34}+q^{34}+A^{10}q^{32}-2A^8q^{32}-4A^6q^{32}+9A^4q^{32}-4A^2q^{32}-10A^6q^{30}+6A^4q^{30}-A^2q^{30}+q^{30}+3A^8q^{28}-4A^6q^{28}+A^4q^{28}+2A^2q^{28}-2q^{28}+A^8q^{26}+A^8q^{26}-8A^4q^{26}-q^{26}+6A^6q^{24}+2A^2q^{24}+q^{24}-A^8q^{22}+4A^6q^{22}-4A^4q^{22}+q^{22}-A^8q^{20}-A^6q^{20}+5A^4q^{20}-6A^2q^{20}+3q^{20}-2A^6q^{18}+8A^4q^{18}-4A^2q^{18}-2q^{18}-3A^6q^{16}+2A^4q^{16}+5A^2q^{16}-2q^{16}-A^6q^{14}-q^{14}-3A^4q^{12}+3A^2q^{12}-2A^4q^{10}-A^2q^{10}+3q^{10}+A^4q^8-4A^2q^8+A^4q^6-A^2q^6-q^2+A^2+1)$                                                                                                                                                                                                                                                                                                                                                                                                                                                                                                                                                                                                                                                                                                                                                                                                                                                                                                                                                                                                                                                                                                                                                                                                                                                                                                                                                                                                                                                                                                                                                                                                                                                                                                                                                                                                                                                                                                                                                                                                                                                                                                                                                                                                                                                                                                                                                                                                                                                                                                                                                                                                                                                                                                                                                                                                                                                                                                                                                                                                                                                                                                                                                                                                                                                                                                                                                                                                                                                                                                                                                                                |

Table 4:  $n^{th}$  differences

| n | c | r | difference                                                                                                                                                                                                                                                                                                                                                                                                                                                                                                                                                                                                                                                                                                                                                                                                                                                                                                                                                                                                                                                                                                                                                                                                                                                                                                                                                                                                                                                                                                                                                                                                                                                                                                                                                                                                                                                                                                                                                                                                                                                                                                                                                                                                                                                                                                                                                                                                                                                                                                                                                                                                                                                                                                                                                                                                                                                                                                                                                                                                                                                                                                                                                                                                                                                                                                                                                                                                                                                                                                                                                                                                                                                                                                                                                                                                                                                                                                                                                                                                                                                                                                                                                                                                                                                                                                                                                                                                                                                                                                                                                                                                                                                                                                                                                                                                                                                                                                                                                                                                                                                                                                                                                                                                                                                                                                                                                                                                                                                                                                                                                                                                                                                                                                                                                                                                                                                                                                                                                                                                                                                                                                                                                                                                                                                                                                                                                                                                                                                                                                                                                                                                                                                                                                                                                                                                                                                                                                                                                                                                                                                                                                                                                                                                                                                                                                                                                                                                                                                                                                                                                                                                                                                                                                                                                                                                                                                                                                                                                                                                                                                                                                                                                                                                                                                                                                                                                                                                                                                                                                                                                                                                                                                                                                                                                                                                                                                                                                                      |
|---|---|---|---------------------------------------------------------------------------------------------------------------------------------------------------------------------------------------------------------------------------------------------------------------------------------------------------------------------------------------------------------------------------------------------------------------------------------------------------------------------------------------------------------------------------------------------------------------------------------------------------------------------------------------------------------------------------------------------------------------------------------------------------------------------------------------------------------------------------------------------------------------------------------------------------------------------------------------------------------------------------------------------------------------------------------------------------------------------------------------------------------------------------------------------------------------------------------------------------------------------------------------------------------------------------------------------------------------------------------------------------------------------------------------------------------------------------------------------------------------------------------------------------------------------------------------------------------------------------------------------------------------------------------------------------------------------------------------------------------------------------------------------------------------------------------------------------------------------------------------------------------------------------------------------------------------------------------------------------------------------------------------------------------------------------------------------------------------------------------------------------------------------------------------------------------------------------------------------------------------------------------------------------------------------------------------------------------------------------------------------------------------------------------------------------------------------------------------------------------------------------------------------------------------------------------------------------------------------------------------------------------------------------------------------------------------------------------------------------------------------------------------------------------------------------------------------------------------------------------------------------------------------------------------------------------------------------------------------------------------------------------------------------------------------------------------------------------------------------------------------------------------------------------------------------------------------------------------------------------------------------------------------------------------------------------------------------------------------------------------------------------------------------------------------------------------------------------------------------------------------------------------------------------------------------------------------------------------------------------------------------------------------------------------------------------------------------------------------------------------------------------------------------------------------------------------------------------------------------------------------------------------------------------------------------------------------------------------------------------------------------------------------------------------------------------------------------------------------------------------------------------------------------------------------------------------------------------------------------------------------------------------------------------------------------------------------------------------------------------------------------------------------------------------------------------------------------------------------------------------------------------------------------------------------------------------------------------------------------------------------------------------------------------------------------------------------------------------------------------------------------------------------------------------------------------------------------------------------------------------------------------------------------------------------------------------------------------------------------------------------------------------------------------------------------------------------------------------------------------------------------------------------------------------------------------------------------------------------------------------------------------------------------------------------------------------------------------------------------------------------------------------------------------------------------------------------------------------------------------------------------------------------------------------------------------------------------------------------------------------------------------------------------------------------------------------------------------------------------------------------------------------------------------------------------------------------------------------------------------------------------------------------------------------------------------------------------------------------------------------------------------------------------------------------------------------------------------------------------------------------------------------------------------------------------------------------------------------------------------------------------------------------------------------------------------------------------------------------------------------------------------------------------------------------------------------------------------------------------------------------------------------------------------------------------------------------------------------------------------------------------------------------------------------------------------------------------------------------------------------------------------------------------------------------------------------------------------------------------------------------------------------------------------------------------------------------------------------------------------------------------------------------------------------------------------------------------------------------------------------------------------------------------------------------------------------------------------------------------------------------------------------------------------------------------------------------------------------------------------------------------------------------------------------------------------------------------------------------------------------------------------------------------------------------------------------------------------------------------------------------------------------------------------------------------------------------------------------------------------------------------------------------------------------------------------------------------------------------------------------------------------------------------------------------------------------------------------------------------------------------------------------------------------------------------------------------------------------------------------------------------------------------------------------------------------------------------------------------------------------------------------------------------------------------------------------------------------------------------------------------------------------------------------------------------------------------------------------------------------------------------------------------------------------------------------------------------------------------------------------------------------------------------------------------------------------------------------------------------------------------------------------------------------------------------------------------------------------------------------------------------------------------------------------------------------------------------------|
| 0 | 5 | 4 | $\begin{aligned} & \frac{A^8}{q^8}(-A^{22}q^{94} + A^{20}q^{94} + A^{24}q^{92} - A^{22}q^{92} + A^{20}q^{92} - A^{18}q^{92} - A^{22}q^{90} + 2A^{20}q^{90} - A^{18}q^{90} - A^{22}q^{88} + A^{16}q^{88} + A^{22}q^{86} - A^{20}q^{84} + \\ & 2A^{18}q^{84} - A^{16}q^{84} - A^{20}q^{82} + A^{14}q^{82} + 2A^{20}q^{80} - A^{18}q^{80} - A^{14}q^{80} - A^{22}q^{78} + A^{20}q^{78} - A^{14}q^{78} + A^{20}q^{76} - 3A^{18}q^{76} + \\ & A^{16}q^{76} + A^{12}q^{76} + A^{20}q^{74} + A^{18}q^{74} - A^{14}q^{74} - A^{20}q^{72} - A^{16}q^{72} + A^{18}q^{72} - A^{12}q^{72} + A^{18}q^{70} - 3A^{16}q^{70} + A^{14}q^{70} + A^{10}q^{70} + \\ & A^{18}q^{68} + A^{16}q^{68} - A^{12}q^{68} - A^{10}q^{68} - A^{18}q^{66} - A^{14}q^{66} + 3A^{12}q^{66} - A^{10}q^{66} + 2A^{14}q^{64} + A^{12}q^{64} + A^{8}q^{64} - A^{18}q^{62} + 3A^{16}q^{62} - \\ & A^{14}q^{62} + A^{12}q^{62} - A^{10}q^{62} - A^{18}q^{60} - A^{18}q^{60} + 2A^{16}q^{60} - 3A^{14}q^{60} + 3A^{10}q^{60} - A^{8}q^{60} - A^{18}q^{58} + 3A^{16}q^{58} + A^{10}q^{58} + A^{6}q^{58} - \\ & A^{18}q^{56} + 3A^{14}q^{56} - 2A^{12}q^{56} - 2A^{10}q^{56} - A^{8}q^{56} - A^{6}q^{56} - A^{16}q^{54} + 3A^{14}q^{54} - 4A^{12}q^{54} + 3A^{10}q^{54} - A^{16}q^{52} + 3A^{14}q^{52} + A^{12}q^{52} - \\ & 6A^{10}q^{52} + 2A^{8}q^{52} + A^{4}q^{52} - A^{16}q^{50} - 3A^{14}q^{50} + 8A^{12}q^{50} - 4A^{10}q^{50} + 2A^{8}q^{50} - A^{6}q^{50} - A^{16}q^{48} + 6A^{14}q^{48} + 8A^{12}q^{48} - 6A^{10}q^{48} - \\ & A^{8}q^{48} + 4A^{6}q^{48} - A^{4}q^{48} + 2A^{16}q^{46} - 6A^{14}q^{46} + 6A^{12}q^{46} + 3A^{10}q^{46} - 8A^{8}q^{46} + 2A^{6}q^{46} + A^{16}q^{44} - 3A^{14}q^{44} - 4A^{12}q^{44} + 11A^{10}q^{44} - \\ & 5A^{8}q^{44} + A^{6}q^{44} - A^{2}q^{44} + A^{16}q^{42} + 2A^{14}q^{42} - 9A^{12}q^{42} + 9A^{10}q^{42} - 3A^{8}q^{42} - 3A^{6}q^{42} + 4A^{4}q^{42} - A^{2}q^{42} + 3A^{14}q^{40} - 6A^{12}q^{40} + 2A^{10}q^{40} + \\ & 8A^{8}q^{40} - 10A^{6}q^{40} + A^{4}q^{40} + A^{2}q^{40} + q^{40} + A^{14}q^{38} - 12A^{10}q^{38} + 16A^{8}q^{38} - 3A^{6}q^{38} - A^{4}q^{38} - q^{38} + 7A^{12}q^{36} - 15A^{10}q^{36} + 9A^{8}q^{36} + A^{6}q^{36} - \\ & 5A^{4}q^{36} + 3A^{2}q^{36} - A^{14}q^{34} + 7A^{12}q^{34} - 8A^{10}q^{34} - 4A^{8}q^{34} + 12A^{6}q^{34} - 6A^{4}q^{34} - A^{2}q^{34} + q^{34} - A^{14}q^{32} + 2A^{12}q^{32} + 3A^{10}q^{32} - 16A^{8}q^{32} + \\ & 13A^{6}q^{32} + 3A^{4}q^{32} - 4A^{2}q^{32} + 10A^{10}q^{30} - 15A^{8}q^{30} - A^{6}q^{30} + 7A^{4}q^{30} - 2A^{2}q^{30} + q^{30} - 2A^{12}q^{28} + 7A^{10}q^{28} - A^{8}q^{28} - 11A^{6}q^{28} + 10A^{4}q^{28} - \\ & A^{2}q^{28} - 2q^{28} - A^{12}q^{26} + 11A^{8}q^{26} - 18A^{6}q^{26} + 2A^{4}q^{26} + 7A^{2}q^{26} - q^{26} - 4A^{10}q^{24} + 14A^{8}q^{24} - 7A^{6}q^{24} + 4A^{4}q^{24} + q^{24} - 4A^{10}q^{22} + \\ & 7A^{8}q^{22} + 7A^{6}q^{22} - 10A^{4}q^{22} - A^{2}q^{22} + q^{22} - 2A^{10}q^{20} - 4A^{8}q^{20} + 13A^{6}q^{20} - 6A^{4}q^{20} - 4A^{2}q^{20} + 3q^{20} - 6A^{8}q^{18} + 10A^{6}q^{18} + 5A^{4}q^{18} - 7A^{2}q^{18} - \\ & 2q^{18} - 4A^{8}q^{16} - A^{6}q^{16} + 9A^{4}q^{16} + A^{2}q^{16} - 2q^{16} - A^{8}q^{14} - 7A^{6}q^{14} + 6A^{4}q^{14} + 3A^{2}q^{14} - q^{14} + 2A^{8}q^{12} - 6A^{6}q^{12} + 4A^{4}q^{12} + A^{8}q^{10} - 2A^{6}q^{10} - \\ & 4A^{4}q^{10} + 2A^{2}q^{10} + 3q^{10} + A^{8}q^8 + A^{6}q^8 - 4A^{4}q^8 - 3A^{2}q^8 + 2A^6q^6 - A^4q^6 - A^2q^6 + A^6q^4 - A^4q^4 - A^2q^4 - q^4 + A^4q^2 - q^2 + A^4 + A^2 + 1) \\ & \frac{A^8}{q^8}(-A^{30}q^{118} + A^{28}q^{118} + A^{32}q^{116} - A^{30}q^{116} + A^{28}q^{116} - A^{26}q^{116} - A^{30}q^{114} + 2A^{28}q^{114} - A^{26}q^{114} - A^{30}q^{112} + A^{24}q^{112} + A^{30}q^{110} - A^{24}q^{110} - \\ & A^{28}q^{108} + 2A^{26}q^{108} - A^{24}q^{108} - A^{28}q^{106} + A^{22}q^{106} + 2A^{28}q^{104} - A^{26}q^{104} - A^{28}q^{102} + A^{28}q^{102} - 2A^{26}q^{102} + 3A^{24}q^{102} - A^{22}q^{102} + \\ & A^{28}q^{100} - 3A^{26}q^{100} + A^{24}q^{100} + A^{20}q^{100} + A^{28}q^{98} + A^{26}q^{98} - A^{22}q^{98} - A^{20}q^{98} - A^{28}q^{96} + A^{24}q^{96} + 3A^{22}q^{96} - A^{20}q^{96} + A^{26}q^{94} - 3A^{24}q^{94} + \\ & A^{22}q^{94} + A^{18}q^{94} + A^{26}q^{92} + A^{24}q^{92} - A^{20}q^{92} - A^{18}q^{92} - A^{26}q^{90} + A^{22}q^{90} + 3A^{20}q^{90} - A^{18}q^{90} + A^{24}q^{88} - 3A^{22}q^{88} + A^{20}q^{88} + A^{16}q^{88} + \\ & A^{24}q^{86} + A^{22}q^{86} - A^{18}q^{86} - A^{16}q^{86} - A^{24}q^{84} - A^{20}q^{84} + 3A^{18}q^{84} - A^{16}q^{84} + A^{22}q^{82} - 3A^{20}q^{82} + A^{18}q^{82} + A^{14}q^{82} + A^{22}q^{80} + A^{20}q^{80} - \\ & A^{16}q^{80} - A^{14}q^{80} - A^{22}q^{78} - A^{18}q^{78} + 3A^{16}q^{78} - A^{14}q^{78} + A^{22}q^{76} - 3A^{18}q^{76} + A^{16}q^{76} + A^{12}q^{76} - A^{24}q^{74} + 2A^{22}q^{74} - A^{20}q^{74} + 2A^{18}q^{74} - \\ & A^{14}q^{74} - A^{12}q^{74} - A^{24}q^{72} + 3A^{22}q^{72} - 4A^{20}q^{72} + A^{18}q^{72} - A^{16}q^{72} + 3A^{14}q^{72} - A^{12}q^{72} - A^{24}q^{70} + 3A^{22}q^{70} - A^{20}q^{70} - 3A^{16}q^{70} + A^{14}q^{70} + \\ & A^{10}q^{70} - A^{24}q^{68} + 2A^{20}q^{68} - 2A^{18}q^{68} + 3A^{16}q^{68} - A^{12}q^{68} - A^{10}q^{68} - A^{22}q^{66} + 4A^{20}q^{66} - 5A^{18}q^{66} + A^{16}q^{66} - A^{14}q^{66} + 3A^{12}q^{66} - A^{10}q^{66} - \\ & A^{22}q^{64} + 3A^{20}q^{64} - 2A^{16}q^{64} - 2A^{14}q^{64} + A^{12}q^{64} + A^{8}q^{64} - A^{22}q^{62} - 3A^{20}q^{62} + 7A^{18}q^{62} - 4A^{16}q^{62} + 3A^{14}q^{62} - A^{10}q^{62} - A^{8}q^{62} + 2A^{22}q^{60} - \\ & 6A^{20}q^{60} + 9A^{18}q^{60} - 7A^{16}q^{60} + 3A^{10}q^{60} - A^{8}q^{60} + 2A^{22}q^{58} - 6A^{20}q^{58} + 6A^{18}q^{58} + 2A^{16}q^{58} - 4A^{14}q^{58} - 2A^{12}q^{58} + A^{10}q^{58} + A^{6}q^{58} + A^{22}q^{56} - \\ & 3A^{20}q^{56} - 4A^{18}q^{56} + 11A^{16}q^{56} - 6A^{14}q^{56} + 2A^{12}q^{56} + A^{10}q^{56} - A^{8}q^{56} - A^{6}q^{56} + A^{22}q^{54} + 2A^{20}q^{54} - 10A^{18}q^{54} + 12A^{16}q^{54} - 5A^{14}q^{54} - \\ & 2A^{12}q^{54} + 3A^{10}q^{54} - A^{6}q^{54} + 3A^{20}q^{52} - 7A^{18}q^{52} + 5A^{16}q^{52} + 5A^{14}q^{52} - 6A^{12}q^{52} - 3A^{10}q^{52} + 2A^{8}q^{52} + A^{4}q^{52} + A^{20}q^{50} - 2A^{18}q^{50} - 9A^{16}q^{50} + \\ & 15A^{14}q^{50} - 4A^{12}q^{50} + A^{8}q^{50} - A^{6}q^{50} - A^{4}q^{50} + 10A^{12}q^{46} - 4A^{10}q^{46} - 5A^{8}q^{46} + 2A^{6}q^{46} + A^{2}q^{46} - A^{20}q^{44} + A^{16}q^{44} - 15A^{14}q^{44} + 17A^{12}q^{44} - \\ & 6A^{18}q^{46} - 8A^{16}q^{46} - A^{14}q^{46} + 10A^{12}q^{42} - 19A^{14}q^{42} + 8A^{12}q^{42} + 3A^{10}q^{42} - 2A^{8}q^{42} - 3A^{6}q^{42} + 4A^{4}q^{42} - A^{2}q^{42} - 2A^{18}q^{40} + 8A^{16}q^{40} - 8A^{14}q^{40} - \\ & A^{10}q^{44} - 2A^{8}q^{44} - A^{2}q^{44} + 10A^{16}q^{42} - 19A^{14}q^{42} + 8A^{12}q^{42} + 3A^{10}q^{42} - 2A^{8}q^{42} - 3A^{6}q^{42} + 4A^{4}q^{42} - A^{2}q^{42} - 2A^{18}q^{38} + 13A^{16}q^{38} + 4A^{8}q^{38} - 2A^{4}q^{38} - \\ & 4A^{12}q^{40} + 11A^{10}q^{40} - A^{8}q^{40} - 7A^{6}q^{40} + A^{4}q^{40} + A^{2}q^{40} + q^{40} - A^{18}q^{38} + 3A^{16}q^{38} + 3A^{14}q^{38} - 19A^{12}q^{38} + 13A^{10}q^{38} + 4A^{8}q^{38} - 2A^{4}q^{38} - \\ & q^{38} - A^{16}q^{36} + 12A^{14}q^{36} - 18A^{12}q^{36} + 3A^{10}q^{36} + 5A^{8}q^{36} + A^{6}q^{36} - 5A^{4}q^{36} + 3A^{2}q^{36} - 2A^{16}q^{34} + 9A^{14}q^{34} - 4A^{12}q^{34} - 11A^{10}q^{34} + 7A^{8}q^{34} + \\ & 6A^{6}q^{34} - 5A^{4}q^{34} - A^{2}q^{34} + q^{34} - A^{16}q^{32} + A^{14}q^{32} + 9A^{12}q^{32} - 20A^{10}q^{32} + 5A^{8}q^{32} + 7A^{6}q^{32} + 3A^{4}q^{32} - 4A^{2}q^{32} - 3A^{14}q^{30} + 18A^{12}q^{30} - \\ & 15A^{10}q^{30} - 7A^{8}q^{30} + 2A^{6}q^{30} + 6A^{4}q^{30} - 2A^{2}q^{30} + q^{30} - 5A^{14}q^{28} + 11A^{12}q^{28} + 3A^{10}q^{28} - 13A^{8}q^{28} + 7A^{4}q^{28} - A^{2}q^{28} - 2q^{28} - 3A^{14}q^{26} + \\ & A^{12}q^{26} + 15A^{10}q^{26} - 14A^{8}q^{26} - 6A^{6}q^{26} + A^{4}q^{26} + 7A^{2}q^{26} - q^{26} - A^{14}q^{24} - 6A^{12}q^{24} + 18A^{10}q^{24} - 3A^{8}q^{24} - 7A^{6}q^{24} - 6A^{4}q^{24} + 4A^{2}q^{24} + \\ & q^{24} - 7A^{12}q^{22} + 7A^{10}q^{22} + 12A^{8}q^{22} - 5A^{6}q^{22} - 7A^{4}q^{22} - A^{2}q^{22} + q^{22} - 3A^{12}q^{20} - 6A^{10}q^{20} + 13A^{8}q^{20} + A^{6}q^{20} - 4A^{4}q^{20} - 4A^{2}q^{20} + 3q^{20} - \\ & 9A^{10}q^{18} + 9A^{8}q^{18} + 7A^{6}q^{18} + 2A^{4}q^{18} - 7A^{2}q^{18} - 2q^{18} + 2A^{12}q^{16} - 7A^{10}q^{16} - 3A^{8}q^{16} + 8A^{6}q^{16} + 5A^{4}q^{16} + A^{2}q^{16} - 2q^{16} + A^{12}q^{14} - A^{10}q^{14} - \\ & 9A^{8}q^{14} + 3A^{6}q^{14} + 4A^{4}q^{14} + 3A^{2}q^{14} - q^{14} + A^{12}q^{12} + 2A^{10}q^{12} - 6A^{8}q^{12} - 2A^{6}q^{12} + A^{4}q^{12} + 4A^{2}q^{12} + 2A^{10}q^{10} - 2A^{8}q^{10} - 4A^{6}q^{10} - A^{4}q^{10} + \\ & 2A^{2}q^{10} + 3q^{10} + A^{10}q^8 + 2A^{8}q^8 - 4A^{6}q^8 - 3A^{4}q^8 - 3A^{2}q^8 + 2A^6q^6 - A^4q^6 - A^2q^6 + A^6q^4 - A^2q^4 - q^4 + A^6q^2 - q^2 + A^6 + A^4 + A^2 + 1) \end{aligned}$ |
| 0 | 7 | 4 | $\begin{aligned} & \frac{A^8}{q^8}(-A^{30}q^{118} + A^{28}q^{118} + A^{32}q^{116} - A^{30}q^{116} + A^{28}q^{116} - A^{26}q^{116} - A^{30}q^{114} + 2A^{28}q^{114} - A^{26}q^{114} - A^{30}q^{112} + A^{24}q^{112} + A^{30}q^{110} - A^{24}q^{110} - \\ & A^{28}q^{108} + 2A^{26}q^{108} - A^{24}q^{108} - A^{28}q^{106} + A^{22}q^{106} + 2A^{28}q^{104} - A^{26}q^{104} - A^{28}q^{102} + A^{28}q^{102} - 2A^{26}q^{102} + 3A^{24}q^{102} - A^{22}q^{102} + \\ & A^{28}q^{100} - 3A^{26}q^{100} + A^{24}q^{100} + A^{20}q^{100} + A^{28}q^{98} + A^{26}q^{98} - A^{22}q^{98} - A^{20}q^{98} - A^{28}q^{96} + A^{24}q^{96} + 3A^{22}q^{96} - A^{20}q^{96} + A^{26}q^{94} - 3A^{24}q^{94} + \\ & A^{22}q^{94} + A^{18}q^{94} + A^{26}q^{92} + A^{24}q^{92} - A^{20}q^{92} - A^{18}q^{92} - A^{26}q^{90} + A^{22}q^{90} + 3A^{20}q^{90} - A^{18}q^{90} + A^{24}q^{88} - 3A^{22}q^{88} + A^{20}q^{88} + A^{16}q^{88} + \\ & A^{24}q^{86} + A^{22}q^{86} - A^{18}q^{86} - A^{16}q^{86} - A^{24}q^{84} - A^{20}q^{84} + 3A^{18}q^{84} - A^{16}q^{84} + A^{22}q^{82} - 3A^{20}q^{82} + A^{18}q^{82} + A^{14}q^{82} + A^{22}q^{80} + A^{20}q^{80} - \\ & A^{16}q^{80} - A^{14}q^{80} - A^{22}q^{78} - A^{18}q^{78} + 3A^{16}q^{78} - A^{14}q^{78} + A^{22}q^{76} - 3A^{18}q^{76} + A^{16}q^{76} + A^{12}q^{76} - A^{24}q^{74} + 2A^{22}q^{74} - A^{20}q^{74} + 2A^{18}q^{74} - \\ & A^{14}q^{74} - A^{12}q^{74} - A^{24}q^{72} + 3A^{22}q^{72} - 4A^{20}q^{72} + A^{18}q^{72} - A^{16}q^{72} + 3A^{14}q^{72} - A^{12}q^{72} - A^{24}q^{70} + 3A^{22}q^{70} - A^{20}q^{70} - 3A^{16}q^{70} + A^{14}q^{70} + \\ & A^{10}q^{70} - A^{24}q^{68} + 2A^{20}q^{68} - 2A^{18}q^{68} + 3A^{16}q^{68} - A^{12}q^{68} - A^{10}q^{68} - A^{22}q^{66} + 4A^{20}q^{66} - 5A^{18}q^{66} + A^{16}q^{66} - A^{14}q^{66} + 3A^{12}q^{66} - A^{10}q^{66} - \\ & A^{22}q^{64} + 3A^{20}q^{64} - 2A^{16}q^{64} - 2A^{14}q^{64} + A^{12}q^{64} + A^{8}q^{64} - A^{22}q^{62} - 3A^{20}q^{62} + 7A^{18}q^{62} - 4A^{16}q^{62} + 3A^{14}q^{62} - A^{10}q^{62} - A^{8}q^{62} + 2A^{22}q^{60} - \\ & 6A^{20}q^{60} + 9A^{18}q^{60} - 7A^{16}q^{60} + 3A^{10}q^{60} - A^{8}q^{60} + 2A^{22}q^{58} - 6A^{20}q^{58} + 6A^{18}q^{58} + 2A^{16}q^{58} - 4A^{14}q^{58} - 2A^{12}q^{58} + A^{10}q^{58} + A^{6}q^{58} + A^{22}q^{56} - \\ & 3A^{20}q^{56} - 4A^{18}q^{56} + 11A^{16}q^{56} - 6A^{14}q^{56} + 2A^{12}q^{56} + A^{10}q^{56} - A^{8}q^{56} - A^{6}q^{56} + A^{22}q^{54} + 2A^{20}q^{54} - 10A^{18}q^{54} + 12A^{16}q^{54} - 5A^{14}q^{54} - \\ & 2A^{12}q^{54} + 3A^{10}q^{54} - A^{6}q^{54} + 3A^{20}q^{52} - 7A^{18}q^{52} + 5A^{16}q^{52} + 5A^{14}q^{52} - 6A^{12}q^{52} - 3A^{10}q^{52} + 2A^{8}q^{52} + A^{4}q^{52} + A^{20}q^{50} - 2A^{18}q^{50} - 9A^{16}q^{50} + \\ & 15A^{14}q^{50} - 4A^{12}q^{50} + A^{8}q^{50} - A^{6}q^{50} - A^{4}q^{50} + 10A^{12}q^{46} - 4A^{10}q^{46} - 5A^{8}q^{46} + 2A^{6}q^{46} + A^{2}q^{46} - A^{20}q^{44} + A^{16}q^{44} - 15A^{14}q^{44} + 17A^{12}q^{44} - \\ & 6A^{18}q^{46} - 8A^{16}q^{46} - A^{14}q^{46} + 10A^{12}q^{42} - 19A^{14}q^{42} + 8A^{12}q^{42} + 3A^{10}q^{42} - 2A^{8}q^{42} - 3A^{6}q^{42} + 4A^{4}q^{42} - A^{2}q^{42} - 2A^{18}q^{40} + 8A^{16}q^{40} - 8A^{14}q^{40} - \\ & A^{10}q^{44} - 2A^{8}q^{44} - A^{2}q^{44} + 10A^{16}q^{42} - 19A^{14}q^{42} + 8A^{12}q^{42} + 3A^{10}q^{42} - 2A^{8}q^{42} - 3A^{6}q^{42} + 4A^{4}q^{42} - A^{2}q^{42} - 2A^{18}q^{38} + 13A^{16}q^{38} + 4A^{8}q^{38} - 2A^{4}q^{38} - \\ & 4A^{12}q^{40} + 11A^{10}q^{40} - A^{8}q^{40} - 7A^{6}q^{40} + A^{4}q^{40} + A^{2}q^{40} + q^{40} - A^{18}q^{38} + 3A^{16}q^{38} + 3A^{14}q^{38} - 19A^{12}q^{38} + 13A^{10}q^{38} + 4A^{8}q^{38} - 2A^{4}q^{38} - \\ & q^{38} - A^{16}q^{36} + 12A^{14}q^{36} - 18A^{12}q^{36} + 3A^{10}q^{36} + 5A^{8}q^{36} + A^{6}q^{36} - 5A^{4}q^{36} + 3A^{2}q^{36} - 2A^{16}q^{34} + 9A^{14}q^{34} - 4A^{12}q^{34} - 11A^{10}q^{34} + 7A^{8}q^{34} + \\ & 6A^{6}q^{34} - 5A^{4}q^{34} - A^{2}q^{34} + q^{34} - A^{16}q^{32} + A^{14}q^{32} + 9A^{12}q^{32} - 20A^{10}q^{32} + 5A^{8}q^{32} + 7A^{6}q^{32} + 3A^{4}q^{32} - 4A^{2}q^{32} - 3A^{14}q^{30} + 18A^{12}q^{30} - \\ & 15A^{10}q^{30} - 7A^{8}q^{30} + 2A^{6}q^{30} + 6A^{4}q^{30} - 2A^{2}q^{30} + q^{30} - 5A^{14}q^{28} + 11A^{12}q^{28} + 3A^{10}q^{28} - 13A^{8}q^{28} + 7A^{4}q^{28} - A^{2}q^{28} - 2q^{28} - 3A^{14}q^{26} + \\ & A^{12}q^{26} + 15A^{10}q^{26} - 14A^{8}q^{26} - 6A^{6}q^{26} + A^{4}q^{26} + 7A^{2}q^{26} - q^{26} - A^{14}q^{24} - 6A^{12}q^{24} + 18A^{10}q^{24} - 3A^{8}q^{24} - 7A^{6}q^{24} - 6A^{4}q^{24} + 4A^{2}q^{24} + \\ & q^{24} - 7A^{12}q^{22} + 7A^{10}q^{22} + 12A^{8}q^{22} - 5A^{6}q^{22} - 7A^{4}q^{22} - A^{2}q^{22} + q^{22} - 3A^{12}q^{20} - 6A^{10}q^{20} + 13A^{8}q^{20} + A^{6}q^{20} - 4A^{4}q^{20} - 4A^{2}q^{20} + 3q^{20} - \\ & 9A^{10}q^{18} + 9A^{8}q^{18} + 7A^{6}q^{18} + 2A^{4}q^{18} - 7A^{2}q^{18} - 2q^{18} + 2A^{12}q^{16} - 7A^{10}q^{16} - 3A^{8}q^{16} + 8A^{6}q^{16} + 5A^{4}q^{16} + A^{2}q^{16} - 2q^{16} + A^{12}q^{14} - A^{10}q^{14} - \\ & 9A^{8}q^{14} + 3A^{6}q^{14} + 4A^{4}q^{14} + 3A^{2}q^{14} - q^{14} + A^{12}q^{12} + 2A^{10}q^{12} - 6A^{8}q^{12} - 2A^{6}q^{12} + A^{4}q^{12} + 4A^{2}q^{12} + 2A^{10}q^{10} - 2A^{8}q^{10} - 4A^{6}q^{10} - A^{4}q^{10} + \\ & 2A^{2}q^{10} + 3q^{10} + A^{10}q^8 + 2A^{8}q^8 - 4A^{6}q^8 - 3A^{4}q^8 - 3A^{2}q^8 + 2A^6q^6 - A^4q^6 - A^2q^6 + A^6q^4 - A^2q^4 - q^4 + A^6q^2 - q^2 + A^6 + A^4 + A^2 + 1) \end{aligned}$                                                                                                                                                                                                                                                                                                                                                                                                                                                                                                                                                                                                                                                                                                                                                                                                                                                                                                                                                                                                                                                                                                                                                                                                                                                                                                                                                                                                                                                                                                                                                                                                                                                                                                                                                                                                                                                                                                                                                                                                                                                                                                                                                                                                                                                                                                                                                                                                                                                                                                                                                                                                                                                                                                                                                                                                                                                                                                                                                                                                                                                                                                                                                                                                                                                                                                                                                                                                                                                               |

Table 5:  $n^{th}$  differences

| n | c | r | difference                                                                                                                                                                                                                                                                                                                                                                                                                                                                                                                                                                                                                                                                                                                                                                                                                                                                                                                                                                                                                                                                                                                                                                                                                                                                                                                                                                                                                                                                                                                                                                                                                                                                                                                                                                                                                                                                                                                                                                                                                                                                                                                                                                                                                                                                                                                                                                                                                                                                                                                                                                                                                                                                                                                                                                                                                                                                                                                                                                                                                                                                                                                                                                                                                                                                                                                                                                                                                                                                                                                                                                                                                                                                                                                                                                                                                                                                                                                                                                                                                                                                                                                                                                                                                                                                                                                                                                                                                                                                                                                                                                                                                                                                                                                                                                                                                                                                                                                                                                                                                                                                                                                                                                                                                                                                                                                                                                                                                                                                                                                                                                                                                                                                                                                                                                                                                                                                                                                                                                                                                                                                                                                                                                                                                                                                                                                                                                                                                                                                                                                                                                                                                                                                                                                                                                                                                                                                                                                                                                                                                                                                                                                                                                                                                                                                                                                                                        |
|---|---|---|-------------------------------------------------------------------------------------------------------------------------------------------------------------------------------------------------------------------------------------------------------------------------------------------------------------------------------------------------------------------------------------------------------------------------------------------------------------------------------------------------------------------------------------------------------------------------------------------------------------------------------------------------------------------------------------------------------------------------------------------------------------------------------------------------------------------------------------------------------------------------------------------------------------------------------------------------------------------------------------------------------------------------------------------------------------------------------------------------------------------------------------------------------------------------------------------------------------------------------------------------------------------------------------------------------------------------------------------------------------------------------------------------------------------------------------------------------------------------------------------------------------------------------------------------------------------------------------------------------------------------------------------------------------------------------------------------------------------------------------------------------------------------------------------------------------------------------------------------------------------------------------------------------------------------------------------------------------------------------------------------------------------------------------------------------------------------------------------------------------------------------------------------------------------------------------------------------------------------------------------------------------------------------------------------------------------------------------------------------------------------------------------------------------------------------------------------------------------------------------------------------------------------------------------------------------------------------------------------------------------------------------------------------------------------------------------------------------------------------------------------------------------------------------------------------------------------------------------------------------------------------------------------------------------------------------------------------------------------------------------------------------------------------------------------------------------------------------------------------------------------------------------------------------------------------------------------------------------------------------------------------------------------------------------------------------------------------------------------------------------------------------------------------------------------------------------------------------------------------------------------------------------------------------------------------------------------------------------------------------------------------------------------------------------------------------------------------------------------------------------------------------------------------------------------------------------------------------------------------------------------------------------------------------------------------------------------------------------------------------------------------------------------------------------------------------------------------------------------------------------------------------------------------------------------------------------------------------------------------------------------------------------------------------------------------------------------------------------------------------------------------------------------------------------------------------------------------------------------------------------------------------------------------------------------------------------------------------------------------------------------------------------------------------------------------------------------------------------------------------------------------------------------------------------------------------------------------------------------------------------------------------------------------------------------------------------------------------------------------------------------------------------------------------------------------------------------------------------------------------------------------------------------------------------------------------------------------------------------------------------------------------------------------------------------------------------------------------------------------------------------------------------------------------------------------------------------------------------------------------------------------------------------------------------------------------------------------------------------------------------------------------------------------------------------------------------------------------------------------------------------------------------------------------------------------------------------------------------------------------------------------------------------------------------------------------------------------------------------------------------------------------------------------------------------------------------------------------------------------------------------------------------------------------------------------------------------------------------------------------------------------------------------------------------------------------------------------------------------------------------------------------------------------------------------------------------------------------------------------------------------------------------------------------------------------------------------------------------------------------------------------------------------------------------------------------------------------------------------------------------------------------------------------------------------------------------------------------------------------------------------------------------------------------------------------------------------------------------------------------------------------------------------------------------------------------------------------------------------------------------------------------------------------------------------------------------------------------------------------------------------------------------------------------------------------------------------------------------------------------------|
| 0 | 9 | 4 | $\begin{aligned} & \frac{A^8}{q^8}(-A^{38}q^{142} + A^{36}q^{142} + A^{40}q^{140} - A^{38}q^{140} + A^{36}q^{140} - A^{34}q^{140} - A^{38}q^{138} + 2A^{36}q^{138} - A^{34}q^{138} - A^{38}q^{136} + A^{32}q^{136} + A^{38}q^{134} - A^{32}q^{134} - \\ & A^{36}q^{132} + 2A^{34}q^{132} - A^{32}q^{132} - A^{36}q^{130} + A^{30}q^{130} + 2A^{36}q^{128} - A^{34}q^{128} - A^{38}q^{126} + A^{36}q^{126} - 2A^{34}q^{126} + 3A^{32}q^{126} - A^{30}q^{126} + \\ & A^{36}q^{124} - 3A^{34}q^{124} + A^{32}q^{124} + A^{28}q^{124} + A^{36}q^{122} + A^{34}q^{122} - A^{30}q^{122} - A^{28}q^{122} - A^{36}q^{120} - A^{32}q^{120} + 3A^{30}q^{120} - A^{28}q^{120} + A^{34}q^{118} - \\ & 3A^{32}q^{118} + A^{30}q^{118} + A^{26}q^{118} + A^{34}q^{116} + A^{32}q^{116} - A^{28}q^{116} - A^{26}q^{116} - A^{34}q^{114} - A^{30}q^{114} + 3A^{28}q^{114} - A^{26}q^{114} + A^{32}q^{112} - 3A^{30}q^{112} + \\ & A^{28}q^{112} + A^{24}q^{112} + A^{32}q^{110} + A^{30}q^{110} - A^{26}q^{110} - A^{24}q^{110} - A^{32}q^{108} - A^{28}q^{108} + 3A^{26}q^{108} - A^{24}q^{108} + A^{30}q^{106} - 3A^{28}q^{106} + A^{26}q^{106} + \\ & A^{22}q^{106} + A^{30}q^{104} + A^{28}q^{104} - A^{24}q^{104} - A^{22}q^{104} - A^{30}q^{102} - A^{26}q^{102} + 3A^{24}q^{102} - A^{22}q^{102} + A^{28}q^{100} - 3A^{26}q^{100} + A^{24}q^{100} + A^{20}q^{100} + \\ & A^{28}q^{98} + A^{26}q^{98} - A^{22}q^{98} - A^{20}q^{98} - A^{28}q^{96} - A^{24}q^{96} + 3A^{22}q^{96} - A^{20}q^{96} + A^{26}q^{94} - 3A^{24}q^{94} + A^{22}q^{94} + A^{18}q^{94} + A^{26}q^{92} + A^{24}q^{92} - A^{20}q^{92} - \\ & A^{18}q^{92} - A^{26}q^{90} - A^{22}q^{90} + 3A^{20}q^{90} - A^{18}q^{90} + A^{28}q^{88} - A^{26}q^{88} + A^{24}q^{88} - 3A^{22}q^{88} + A^{20}q^{88} + A^{16}q^{88} - A^{30}q^{86} + 2A^{28}q^{86} + \\ & 2A^{24}q^{86} + A^{22}q^{86} - A^{18}q^{86} - A^{16}q^{86} - A^{30}q^{84} + 3A^{28}q^{84} - 3A^{26}q^{84} - A^{20}q^{84} + 3A^{18}q^{84} - A^{16}q^{84} - A^{30}q^{82} + 3A^{28}q^{82} - A^{26}q^{82} - A^{24}q^{82} + \\ & A^{22}q^{82} - 3A^{20}q^{82} + A^{18}q^{82} + A^{14}q^{78} - A^{14}q^{78} - A^{28}q^{76} + 3A^{26}q^{76} - 3A^{24}q^{76} + 2A^{20}q^{76} - 3A^{18}q^{76} + A^{16}q^{76} + A^{12}q^{76} - A^{28}q^{74} - 3A^{26}q^{74} + \\ & A^{18}q^{78} + 3A^{16}q^{78} - A^{14}q^{74} - A^{14}q^{74} - A^{12}q^{74} + 2A^{28}q^{72} - 6A^{26}q^{72} + 9A^{24}q^{72} - 6A^{22}q^{72} - A^{20}q^{72} + A^{18}q^{72} - A^{16}q^{72} + 3A^{14}q^{72} - A^{12}q^{72} + 2A^{28}q^{70} - \\ & 3A^{20}q^{74} + A^{18}q^{74} - A^{14}q^{74} - A^{12}q^{74} + 2A^{28}q^{72} - 6A^{26}q^{72} + 9A^{24}q^{72} - 6A^{22}q^{72} - A^{20}q^{72} + A^{18}q^{72} - A^{16}q^{72} + 3A^{14}q^{72} - A^{12}q^{72} + 2A^{28}q^{70} - \\ & 6A^{26}q^{70} + 6A^{24}q^{70} + 2A^{22}q^{70} - 5A^{20}q^{70} + 2A^{18}q^{70} - 3A^{16}q^{70} + A^{14}q^{70} + A^{10}q^{70} + A^{28}q^{68} - 3A^{26}q^{68} - 4A^{24}q^{68} + 11A^{22}q^{68} - 7A^{20}q^{68} + 2A^{18}q^{68} + \\ & 2A^{16}q^{68} - A^{12}q^{68} - A^{10}q^{68} + A^{28}q^{66} + 2A^{26}q^{66} - 10A^{24}q^{66} + 12A^{22}q^{66} - 4A^{20}q^{66} - 3A^{18}q^{66} + A^{16}q^{66} - A^{14}q^{66} + 3A^{12}q^{66} - A^{10}q^{66} + 3A^{26}q^{64} - \\ & 7A^{24}q^{64} + 5A^{22}q^{64} + 5A^{20}q^{64} - 7A^{18}q^{64} + A^{16}q^{64} - 2A^{14}q^{64} + A^{12}q^{64} + A^{8}q^{64} + A^{26}q^{62} - 2A^{24}q^{62} - 9A^{22}q^{62} + 15A^{20}q^{62} - 5A^{18}q^{62} + 2A^{14}q^{62} - \\ & A^{10}q^{62} - A^{8}q^{62} + 6A^{24}q^{60} - 14A^{22}q^{60} + 12A^{20}q^{60} - A^{18}q^{60} - 5A^{16}q^{60} + 3A^{10}q^{60} - A^{8}q^{60} - A^{26}q^{58} + 6A^{24}q^{58} - 9A^{22}q^{58} + A^{20}q^{58} + 9A^{18}q^{58} - \\ & 5A^{16}q^{58} - A^{14}q^{58} - 2A^{12}q^{58} + A^{10}q^{58} + A^{6}q^{58} - A^{26}q^{56} + 2A^{24}q^{56} - 12A^{20}q^{56} + 15A^{18}q^{56} - 2A^{16}q^{56} - 2A^{14}q^{56} + A^{12}q^{56} + A^{10}q^{56} - A^{8}q^{56} - \\ & A^{6}q^{56} + 8A^{22}q^{54} - 16A^{20}q^{54} + 8A^{18}q^{54} + 3A^{16}q^{54} - 3A^{14}q^{54} - 2A^{12}q^{54} - A^{6}q^{54} - 2A^{24}q^{52} + 7A^{22}q^{52} - 7A^{20}q^{52} - 3A^{18}q^{52} - 10A^{16}q^{52} - \\ & 2A^{14}q^{52} - 3A^{12}q^{52} - 3A^{10}q^{52} + 2A^{8}q^{52} + A^{4}q^{52} - A^{24}q^{50} + 2A^{22}q^{50} + 3A^{20}q^{50} - 16A^{18}q^{50} + 12A^{16}q^{50} + 2A^{14}q^{50} - A^{10}q^{50} + A^{8}q^{50} - A^{6}q^{50} - \\ & A^{4}q^{50} - A^{22}q^{48} + 10A^{20}q^{48} - 17A^{18}q^{48} + 7A^{16}q^{48} + 3A^{14}q^{48} - 4A^{10}q^{48} - A^{8}q^{48} + 4A^{6}q^{48} - A^{4}q^{48} - 2A^{22}q^{46} + 9A^{20}q^{46} - 8A^{18}q^{46} - 4A^{16}q^{46} + \\ & 6A^{14}q^{46} + 2A^{12}q^{46} - A^{10}q^{46} - 5A^{8}q^{46} + 2A^{6}q^{46} + A^{2}q^{46} - A^{22}q^{44} + 2A^{20}q^{44} + 2A^{18}q^{44} - 14A^{16}q^{44} + 10A^{14}q^{44} + 2A^{12}q^{44} + 3A^{10}q^{44} - 3A^{8}q^{44} - \\ & A^{2}q^{44} + 10A^{18}q^{42} - 17A^{16}q^{42} + 5A^{14}q^{42} + 4A^{10}q^{42} - 2A^{8}q^{42} - 3A^{6}q^{42} + 4A^{4}q^{42} - A^{2}q^{42} - 2A^{20}q^{40} + 9A^{18}q^{40} - 8A^{16}q^{40} - 4A^{14}q^{40} + 5A^{12}q^{40} + \\ & 2A^{10}q^{40} + 2A^{8}q^{40} - 7A^{6}q^{40} + A^{4}q^{40} + A^{2}q^{40} - A^{20}q^{38} + 3A^{18}q^{38} + 4A^{16}q^{38} - 17A^{14}q^{38} + 8A^{12}q^{38} + 7A^{10}q^{38} - A^{6}q^{38} - 2A^{4}q^{38} - A^{18}q^{36} + \\ & 14A^{16}q^{36} - 19A^{14}q^{36} + 3A^{12}q^{36} - A^{10}q^{36} + 5A^{8}q^{36} + A^{6}q^{36} - 5A^{4}q^{36} + 3A^{2}q^{36} - 4A^{18}q^{34} + 15A^{16}q^{34} - 7A^{14}q^{34} - 9A^{12}q^{34} + 2A^{10}q^{34} + A^{8}q^{34} + \\ & 7A^{6}q^{34} - 5A^{4}q^{34} - A^{2}q^{34} + q^{34} - 4A^{18}q^{32} + 6A^{16}q^{32} + 9A^{14}q^{32} - 19A^{12}q^{32} + 3A^{10}q^{32} - A^{8}q^{32} + 7A^{6}q^{32} + 3A^{4}q^{32} - 4A^{2}q^{32} - 2A^{18}q^{30} - A^{16}q^{30} + \\ & 20A^{14}q^{30} - 14A^{12}q^{30} - 5A^{10}q^{30} - 4A^{8}q^{30} + A^{6}q^{30} + 6A^{4}q^{30} - 2A^{2}q^{30} + q^{30} - A^{18}q^{28} - 7A^{16}q^{28} + 16A^{14}q^{28} + 3A^{12}q^{28} - 10A^{10}q^{28} - 2A^{8}q^{28} - \\ & 3A^{6}q^{28} + 7A^{4}q^{28} - A^{2}q^{28} - 2q^{28} - 6A^{16}q^{26} + 2A^{14}q^{26} + 18A^{12}q^{26} - 12A^{10}q^{26} - 2A^{8}q^{26} - 7A^{6}q^{26} + A^{4}q^{26} + 7A^{2}q^{26} - q^{26} - 2A^{16}q^{24} - 8A^{14}q^{24} + \\ & 19A^{12}q^{24} - 3A^{8}q^{24} - 5A^{6}q^{24} - 6A^{4}q^{24} + 4A^{2}q^{24} + q^{24} - 10A^{14}q^{22} + 7A^{12}q^{22} + 12A^{10}q^{22} - 2A^{8}q^{22} - 7A^{6}q^{22} - A^{2}q^{22} + q^{22} + 2A^{16}q^{20} - 6A^{14}q^{20} - \\ & 8A^{12}q^{20} + 13A^{10}q^{20} + A^{8}q^{20} + 3A^{6}q^{20} - 4A^{4}q^{20} - 4A^{2}q^{20} + 3q^{20} + A^{16}q^{18} - 11A^{12}q^{18} + 7A^{10}q^{18} + 6A^{8}q^{18} + 4A^{6}q^{18} + 2A^{4}q^{18} - 7A^{2}q^{18} - 2q^{18} + \\ & A^{16}q^{16} + 2A^{14}q^{16} - 7A^{12}q^{16} - 5A^{10}q^{16} + 6A^{8}q^{16} + 4A^{6}q^{16} + A^{2}q^{16} - 2q^{16} + 2A^{14}q^{14} - A^{12}q^{14} - 9A^{10}q^{14} + A^{8}q^{14} + A^{6}q^{14} + 4A^{4}q^{14} + \\ & 3A^{2}q^{14} - q^{14} + A^{14}q^{12} + 3A^{12}q^{12} - 6A^{10}q^{12} - 2A^{8}q^{12} - A^{6}q^{12} + A^{4}q^{12} + 4A^{2}q^{12} + 2A^{12}q^{10} - A^{10}q^{10} - 4A^{8}q^{10} - A^{6}q^{10} - A^{4}q^{10} + 2A^{2}q^{10} + 3q^{10} + \\ & A^{12}q^8 + 2A^{10}q^8 - 3A^8q^8 - 3A^6q^8 - 3A^4q^8 - 3A^2q^8 + 2A^{10}q^6 - A^4q^6 - A^2q^6 + A^{10}q^4 + A^8q^4 - A^2q^4 - q^4 + A^8q^2 - q^2 + A^8 + A^6 + A^4 + A^2 + 1) \end{aligned}$ |

Table 6:  $n^{th}$  differences

| n | c  | r | difference                                                                                                                                                                                                                                                                                                                                                                                                                                                                                                                                                                                                                                                                                                                                                                                                                                                                                                                                                                                                                                                                                                                                                                                                                                                                                                                                                                                                                                                                                                                                                                                                                                                                                                                                                                                                                                                                                                                                                                                                                                                                                                                                                                                                                                                                                                                                                                                                                                                                                                                                                                                                                                                                                                                                                                                                                                                                                                                                                                                                                                                                                                                                                                                                                                                                                                                                                                                                                                                                                                                                                                                                                                                                                                                                                                                                                                                                                                                                                                                                                                                                                                                                                                                                                                                                                                                                                                                                                                                                                                                                                                                                                                                                                                                                                                                                                                                                                                                                                                                                                                                                                                                                                                                                                                                                                                                                                                                                                                                                                                                                                                                                                                                                                                                                                                                                                                                                                                                                                                                                                                                                                                                                                                                                                                                                                                                                                                                                                                                                                                                                                                                                                                                                                                                                                                                                                                                                                                                                                                                                                                                                                                                                                                                                                                                                                                                                                                                                                                                                                                                                                                                                                                                                                                                                                                                                                                                                                                                                                                                                                                                                                                                                                                                                                                                                                                                                                                                                                                                                                                                                                                                                                                                                                                                                                                                                                                                                                                                                                                                                                                                                                                                                                                                                                                                                                                                                                                                                                                                                                                  |
|---|----|---|-------------------------------------------------------------------------------------------------------------------------------------------------------------------------------------------------------------------------------------------------------------------------------------------------------------------------------------------------------------------------------------------------------------------------------------------------------------------------------------------------------------------------------------------------------------------------------------------------------------------------------------------------------------------------------------------------------------------------------------------------------------------------------------------------------------------------------------------------------------------------------------------------------------------------------------------------------------------------------------------------------------------------------------------------------------------------------------------------------------------------------------------------------------------------------------------------------------------------------------------------------------------------------------------------------------------------------------------------------------------------------------------------------------------------------------------------------------------------------------------------------------------------------------------------------------------------------------------------------------------------------------------------------------------------------------------------------------------------------------------------------------------------------------------------------------------------------------------------------------------------------------------------------------------------------------------------------------------------------------------------------------------------------------------------------------------------------------------------------------------------------------------------------------------------------------------------------------------------------------------------------------------------------------------------------------------------------------------------------------------------------------------------------------------------------------------------------------------------------------------------------------------------------------------------------------------------------------------------------------------------------------------------------------------------------------------------------------------------------------------------------------------------------------------------------------------------------------------------------------------------------------------------------------------------------------------------------------------------------------------------------------------------------------------------------------------------------------------------------------------------------------------------------------------------------------------------------------------------------------------------------------------------------------------------------------------------------------------------------------------------------------------------------------------------------------------------------------------------------------------------------------------------------------------------------------------------------------------------------------------------------------------------------------------------------------------------------------------------------------------------------------------------------------------------------------------------------------------------------------------------------------------------------------------------------------------------------------------------------------------------------------------------------------------------------------------------------------------------------------------------------------------------------------------------------------------------------------------------------------------------------------------------------------------------------------------------------------------------------------------------------------------------------------------------------------------------------------------------------------------------------------------------------------------------------------------------------------------------------------------------------------------------------------------------------------------------------------------------------------------------------------------------------------------------------------------------------------------------------------------------------------------------------------------------------------------------------------------------------------------------------------------------------------------------------------------------------------------------------------------------------------------------------------------------------------------------------------------------------------------------------------------------------------------------------------------------------------------------------------------------------------------------------------------------------------------------------------------------------------------------------------------------------------------------------------------------------------------------------------------------------------------------------------------------------------------------------------------------------------------------------------------------------------------------------------------------------------------------------------------------------------------------------------------------------------------------------------------------------------------------------------------------------------------------------------------------------------------------------------------------------------------------------------------------------------------------------------------------------------------------------------------------------------------------------------------------------------------------------------------------------------------------------------------------------------------------------------------------------------------------------------------------------------------------------------------------------------------------------------------------------------------------------------------------------------------------------------------------------------------------------------------------------------------------------------------------------------------------------------------------------------------------------------------------------------------------------------------------------------------------------------------------------------------------------------------------------------------------------------------------------------------------------------------------------------------------------------------------------------------------------------------------------------------------------------------------------------------------------------------------------------------------------------------------------------------------------------------------------------------------------------------------------------------------------------------------------------------------------------------------------------------------------------------------------------------------------------------------------------------------------------------------------------------------------------------------------------------------------------------------------------------------------------------------------------------------------------------------------------------------------------------------------------------------------------------------------------------------------------------------------------------------------------------------------------------------------------------------------------------------------------------------------------------------------------------------------------------------------------------------------------------------------------------------------------------------------------------------------------------------------------------------------------------------------------------------------------------------------------------------------------------------------------------------------------------------------------------------------------------------------------------------------------------------------------------------------------------------------------------------------------------------------------------------------------------------------------------------------------------------------------------------------------------------------------------------------------------------------------------------------------------------------------------------------------------------------------------------------------------------------------------------------------------------------------------------------------------------------------------------------------------------------------------------------------------------------------------------------------------------------------|
| 0 | 11 | 4 | $\begin{aligned} & \frac{A^8}{q^8} (-A^{46}q^{166} + A^{44}q^{166} + A^{48}q^{164} - A^{46}q^{164} + A^{44}q^{164} - A^{42}q^{164} - A^{46}q^{162} + 2A^{44}q^{162} - A^{42}q^{162} - A^{46}q^{160} + A^{40}q^{160} + A^{46}q^{158} - A^{40}q^{158} - \\ & A^{44}q^{156} + 2A^{42}q^{156} - A^{40}q^{156} - A^{44}q^{154} + A^{38}q^{154} + 2A^{44}q^{152} - A^{42}q^{152} - A^{46}q^{150} + A^{44}q^{150} - 2A^{42}q^{150} + 3A^{40}q^{150} + \\ & A^{44}q^{148} - 3A^{42}q^{148} + A^{40}q^{148} + A^{36}q^{148} + A^{44}q^{146} + A^{42}q^{146} - A^{36}q^{146} - A^{44}q^{144} - A^{40}q^{144} + 3A^{38}q^{144} - A^{36}q^{144} + A^{42}q^{142} - \\ & 3A^{40}q^{142} + A^{38}q^{142} + A^{34}q^{142} + A^{42}q^{140} + A^{40}q^{140} - A^{36}q^{140} - A^{34}q^{140} - A^{42}q^{138} - A^{38}q^{138} - A^{34}q^{138} + A^{40}q^{136} - 3A^{38}q^{136} + \\ & A^{36}q^{136} + A^{32}q^{136} + A^{40}q^{134} + A^{38}q^{134} - A^{34}q^{134} - A^{32}q^{134} - A^{40}q^{132} - A^{36}q^{132} + 3A^{34}q^{132} - A^{32}q^{132} + A^{38}q^{130} - 3A^{36}q^{130} + A^{34}q^{130} + \\ & A^{30}q^{130} + A^{38}q^{128} + A^{36}q^{128} - A^{32}q^{128} - A^{30}q^{128} - A^{38}q^{126} - A^{34}q^{126} + 3A^{32}q^{126} - A^{30}q^{126} + A^{36}q^{124} - 3A^{34}q^{124} + A^{32}q^{124} + A^{28}q^{124} + \\ & A^{36}q^{122} + A^{34}q^{122} - A^{30}q^{122} - A^{28}q^{122} - A^{36}q^{120} - A^{32}q^{120} + 3A^{30}q^{120} - A^{28}q^{120} + A^{34}q^{118} - 3A^{32}q^{118} + A^{30}q^{118} + A^{26}q^{118} + A^{34}q^{116} + \\ & A^{32}q^{116} - A^{28}q^{116} - A^{26}q^{116} - A^{34}q^{114} - A^{30}q^{114} + 3A^{28}q^{114} - A^{26}q^{114} + A^{32}q^{112} - 3A^{30}q^{112} + A^{28}q^{112} + A^{24}q^{112} + A^{32}q^{110} + A^{30}q^{110} - \\ & A^{26}q^{110} - A^{24}q^{110} - A^{32}q^{108} - A^{28}q^{108} + 3A^{26}q^{108} - A^{24}q^{108} + A^{30}q^{106} - 3A^{28}q^{106} + A^{26}q^{106} + A^{22}q^{106} + A^{30}q^{104} + A^{28}q^{104} - A^{24}q^{104} - \\ & A^{22}q^{104} - A^{30}q^{102} - A^{26}q^{102} + 3A^{24}q^{102} - A^{22}q^{102} + A^{34}q^{100} - A^{32}q^{100} + A^{28}q^{100} - 3A^{26}q^{100} + A^{24}q^{100} + A^{20}q^{100} - A^{36}q^{98} + 2A^{34}q^{98} - \\ & 2A^{32}q^{98} + A^{30}q^{98} + A^{28}q^{98} + A^{26}q^{98} - A^{22}q^{98} - A^{20}q^{98} - A^{36}q^{96} + 3A^{34}q^{96} - A^{32}q^{96} + A^{30}q^{96} - A^{28}q^{96} - A^{24}q^{96} - A^{20}q^{96} - A^{36}q^{94} + \\ & 3A^{34}q^{94} - A^{32}q^{94} - A^{30}q^{94} + A^{26}q^{94} - 3A^{24}q^{94} + A^{22}q^{94} + A^{18}q^{94} - A^{36}q^{92} + 2A^{32}q^{92} - 3A^{30}q^{92} + 2A^{28}q^{92} + A^{26}q^{92} + A^{24}q^{92} - A^{20}q^{92} - \\ & A^{18}q^{92} - A^{34}q^{90} + 4A^{32}q^{90} - 4A^{30}q^{90} + A^{28}q^{90} - A^{26}q^{90} - A^{22}q^{90} + 3A^{20}q^{90} - A^{18}q^{90} - A^{34}q^{88} + 3A^{32}q^{88} - 3A^{28}q^{88} + A^{26}q^{88} + A^{24}q^{88} - \\ & 3A^{22}q^{88} + A^{20}q^{88} + A^{16}q^{88} - A^{34}q^{86} - 3A^{32}q^{86} + 7A^{30}q^{86} - 5A^{28}q^{86} + 2A^{26}q^{86} + A^{24}q^{86} + A^{22}q^{86} - A^{18}q^{86} - A^{16}q^{86} + 2A^{34}q^{84} - 6A^{32}q^{84} + \\ & 9A^{30}q^{84} - 6A^{28}q^{84} - A^{20}q^{84} + 3A^{18}q^{84} - A^{16}q^{84} + 2A^{34}q^{82} - 6A^{32}q^{82} + 6A^{30}q^{82} + 2A^{28}q^{82} - 5A^{26}q^{82} + A^{24}q^{82} + A^{22}q^{82} - 3A^{20}q^{82} + A^{18}q^{82} + \\ & A^{14}q^{82} + A^{34}q^{80} - 3A^{32}q^{80} - 4A^{30}q^{80} + 11A^{28}q^{80} - 7A^{26}q^{80} + A^{24}q^{80} + 2A^{22}q^{80} + A^{20}q^{80} - A^{16}q^{80} - A^{14}q^{80} + A^{34}q^{78} + 2A^{32}q^{78} - 10A^{30}q^{78} + \\ & 12A^{28}q^{78} - 4A^{26}q^{78} - 2A^{24}q^{78} - A^{18}q^{78} + 3A^{16}q^{78} - A^{14}q^{78} + 3A^{32}q^{76} - 7A^{30}q^{76} + 5A^{28}q^{76} + 5A^{26}q^{76} - 7A^{24}q^{76} + 2A^{20}q^{76} - 3A^{18}q^{76} + \\ & A^{16}q^{76} + A^{12}q^{76} + A^{32}q^{74} - 2A^{30}q^{74} - 9A^{28}q^{74} + 15A^{26}q^{74} - 5A^{24}q^{74} - A^{22}q^{74} + 2A^{20}q^{74} + A^{18}q^{74} - A^{14}q^{74} - A^{12}q^{74} + 6A^{30}q^{72} - 14A^{28}q^{72} + \\ & 12A^{26}q^{72} - A^{24}q^{72} - 4A^{22}q^{72} - A^{20}q^{72} + A^{18}q^{72} + 3A^{14}q^{72} - A^{12}q^{72} - A^{32}q^{70} + 6A^{30}q^{70} - 9A^{28}q^{70} + A^{26}q^{70} + 9A^{24}q^{70} - 5A^{22}q^{70} - \\ & 2A^{20}q^{70} + 2A^{18}q^{70} - 3A^{16}q^{70} + A^{14}q^{70} + A^{10}q^{70} - A^{32}q^{68} + 2A^{30}q^{68} - 12A^{26}q^{68} + 15A^{24}q^{68} - 2A^{22}q^{68} - 3A^{20}q^{68} + A^{18}q^{68} + 2A^{16}q^{68} - A^{12}q^{68} - \\ & A^{10}q^{68} + 8A^{28}q^{66} - 16A^{26}q^{66} + 8A^{24}q^{66} + 3A^{22}q^{66} - 2A^{20}q^{66} - 3A^{18}q^{66} + A^{16}q^{66} + A^{14}q^{66} - A^{10}q^{66} - 2A^{30}q^{64} + 7A^{28}q^{64} - 7A^{26}q^{64} - \\ & 2A^{24}q^{64} + 9A^{22}q^{64} - 2A^{20}q^{64} - 4A^{18}q^{64} + A^{16}q^{64} - 2A^{14}q^{64} + A^{12}q^{64} + A^{8}q^{64} - A^{30}q^{62} + 2A^{28}q^{62} + 2A^{26}q^{62} - 14A^{24}q^{62} + 11A^{22}q^{62} + 2A^{20}q^{62} - \\ & A^{18}q^{62} - A^{16}q^{62} + 2A^{14}q^{62} - A^{10}q^{62} - A^{8}q^{62} - A^{28}q^{60} + 9A^{26}q^{60} - 14A^{24}q^{60} + 5A^{22}q^{60} + 3A^{20}q^{60} + A^{18}q^{60} - 5A^{16}q^{60} + 3A^{10}q^{60} - A^{8}q^{60} - \\ & 2A^{28}q^{58} + 7A^{26}q^{58} - 5A^{24}q^{58} - 4A^{22}q^{58} + 5A^{20}q^{58} + 2A^{18}q^{58} - 2A^{16}q^{58} - A^{14}q^{58} - 2A^{12}q^{58} + A^{10}q^{58} - A^{8}q^{58} - A^{26}q^{56} + 3A^{24}q^{56} - \\ & 13A^{22}q^{56} + 9A^{20}q^{56} + 2A^{18}q^{56} + 2A^{16}q^{56} - 3A^{14}q^{56} + A^{12}q^{56} + A^{10}q^{56} - A^{8}q^{56} - A^{26}q^{54} + 10A^{24}q^{54} - 14A^{22}q^{54} + 4A^{20}q^{54} - A^{18}q^{54} + \\ & 5A^{16}q^{54} - 3A^{14}q^{54} - 2A^{12}q^{54} + 3A^{8}q^{54} - A^{6}q^{54} - 2A^{26}q^{52} + 7A^{24}q^{52} - 7A^{22}q^{52} + 2A^{18}q^{52} + A^{14}q^{52} - 3A^{12}q^{52} - 3A^{10}q^{52} + 2A^{8}q^{52} + \\ & A^{4}q^{52} - A^{26}q^{50} + 3A^{24}q^{50} - 10A^{20}q^{50} + 7A^{18}q^{50} - 2A^{16}q^{50} + 6A^{14}q^{50} - A^{12}q^{50} - A^{10}q^{50} + A^{8}q^{50} - A^{6}q^{50} - A^{4}q^{50} + 7A^{22}q^{48} - 13A^{20}q^{48} + \\ & 7A^{18}q^{48} - 4A^{16}q^{48} + 5A^{14}q^{48} - 4A^{10}q^{48} - A^{8}q^{48} + 4A^{6}q^{48} - A^{4}q^{48} - A^{24}q^{46} + 7A^{22}q^{46} - 9A^{20}q^{46} + 2A^{18}q^{46} + A^{16}q^{46} - 2A^{14}q^{46} + 5A^{12}q^{46} - \\ & A^{10}q^{46} - 5A^{8}q^{46} + 2A^{6}q^{46} + A^{2}q^{46} - A^{24}q^{44} + 4A^{22}q^{44} - 2A^{20}q^{44} - 11A^{18}q^{44} + 11A^{16}q^{44} - 5A^{14}q^{44} + 6A^{12}q^{44} + 2A^{10}q^{44} - 3A^{8}q^{44} - A^{2}q^{44} + \\ & A^{22}q^{42} + 9A^{20}q^{42} - 18A^{18}q^{42} + 9A^{16}q^{42} - 4A^{14}q^{42} + A^{12}q^{42} + 4A^{10}q^{42} - 2A^{8}q^{42} - 3A^{6}q^{42} + 4A^{4}q^{42} - A^{2}q^{42} - 2A^{22}q^{40} + 12A^{20}q^{40} - 13A^{18}q^{40} - \\ & A^{16}q^{40} + 5A^{14}q^{40} - 4A^{12}q^{40} + 5A^{10}q^{40} + 2A^{8}q^{40} - 7A^{6}q^{40} + A^{4}q^{40} + A^{2}q^{40} + q^{40} - 3A^{22}q^{38} + 10A^{20}q^{38} - A^{18}q^{38} - 18A^{16}q^{38} + 12A^{14}q^{38} - \\ & 5A^{12}q^{38} + 3A^{10}q^{38} + 6A^{8}q^{38} - A^{6}q^{38} - 2A^{4}q^{38} - q^{38} - 3A^{22}q^{36} + 4A^{20}q^{36} + 15A^{18}q^{36} - 22A^{16}q^{36} + 4A^{14}q^{36} - A^{12}q^{36} - A^{10}q^{36} + 5A^{8}q^{36} + \\ & A^{6}q^{36} - 5A^{4}q^{36} + 3A^{2}q^{36} - 2A^{22}q^{34} - 2A^{20}q^{34} + 18A^{18}q^{34} - 8A^{16}q^{34} - 10A^{14}q^{34} + 4A^{12}q^{34} - 4A^{10}q^{34} + 2A^{8}q^{34} + 7A^{6}q^{34} - 5A^{4}q^{34} - A^{2}q^{34} + \\ & q^{34} - A^{22}q^{32} - 6A^{20}q^{32} + 11A^{18}q^{32} + 10A^{16}q^{32} - 20A^{14}q^{32} + 4A^{12}q^{32} - 3A^{10}q^{32} - A^{8}q^{32} + 7A^{6}q^{32} + 3A^{4}q^{32} - 4A^{2}q^{32} - 5A^{20}q^{30} + 24A^{16}q^{30} - \\ & 14A^{14}q^{30} - 4A^{12}q^{30} - 2A^{10}q^{30} - 5A^{8}q^{30} + A^{6}q^{30} + 6A^{4}q^{30} - 2A^{2}q^{30} + q^{30} - 2A^{20}q^{28} - 9A^{18}q^{28} + 17A^{16}q^{28} + 7A^{14}q^{28} - 10A^{12}q^{28} + A^{10}q^{28} - \\ & 5A^{8}q^{28} - 3A^{6}q^{28} + 7A^{4}q^{28} - A^{2}q^{28} - 2Q^{28} - 9A^{18}q^{26} + 2A^{16}q^{26} + 19A^{14}q^{26} - 9A^{12}q^{26} - 3A^{8}q^{26} - 7A^{6}q^{26} + A^{4}q^{26} + 7A^{2}q^{26} - q^{26} + 2A^{20}q^{24} - \\ & 5A^{18}q^{24} - 10A^{16}q^{24} + 19A^{14}q^{24} + A^{12}q^{24} - A^{8}q^{24} - 5A^{6}q^{24} - 6A^{4}q^{24} + 4A^{2}q^{24} + q^{24} + A^{20}q^{22} - 12A^{16}q^{22} + 5A^{14}q^{22} + 12A^{12}q^{22} + 3A^{8}q^{22} - \\ & 2A^{6}q^{22} - 7A^{4}q^{22} - A^{2}q^{22} + q^{22} + A^{20}q^{20} + 2A^{18}q^{20} - 6A^{16}q^{20} - 10A^{14}q^{20} - 10A^{12}q^{20} + 11A^{12}q^{20} + A^{10}q^{20} + 3A^{8}q^{20} + 3A^{6}q^{20} - 4A^{4}q^{20} - 4A^{2}q^{20} + 3q^{20} + \\ & 2A^{18}q^{18} - 11A^{14}q^{18} + 5A^{12}q^{18} + 4A^{10}q^{18} + 3A^{8}q^{18} + 4A^{6}q^{18} + 2A^{4}q^{18} - 7A^{2}q^{18} - 2Q^{18} + A^{18}q^{16} + 3A^{16}q^{16} - 7A^{14}q^{16} - 5A^{12}q^{16} + 4A^{10}q^{16} + \\ & 2A^{8}q^{16} + 4A^{6}q^{16} + 5A^{4}q^{16} + A^{2}q^{16} - 2Q^{16} + 2A^{16}q^{14} - 9A^{12}q^{14} + A^{10}q^{14} - A^{8}q^{14} + A^{6}q^{14} + 4A^{4}q^{14} + 3A^{2}q^{14} - q^{14} + A^{16}q^{12} + 3A^{14}q^{12} - \\ & 5A^{12}q^{12} - 2A^{10}q^{12} - A^{8}q^{12} - A^{6}q^{12} + A^{4}q^{12} + 4A^{2}q^{12} + 2A^{14}q^{10} - A^{12}q^{10} - 3A^{10}q^{10} - A^{8}q^{10} - A^{6}q^{10} - 2A^{2}q^{10} + 3q^{10} + A^{14}q^8 + 2A^{12}q^8 - \\ & 3A^{10}q^8 - 2A^{8}q^8 - 3A^{6}q^8 - 3A^{4}q^8 - 3A^{2}q^8 + 2A^{12}q^6 - A^{4}q^6 - A^{2}q^6 + A^{12}q^4 + A^{10}q^4 - A^{2}q^4 - q^4 + A^{10}q^2 - q^2 + A^{10} + A^8 + A^6 + A^4 + A^2 + 1) \end{aligned}$ |

Table 7:  $n^{th}$  differences



## $n^{\text{th}}$ Differences of $F$ -Factors

The  $n^{\text{th}}$  differences of  $F$ -factors also seem to have many quantum numbers as factors. While we do not prove here a similar result as we did before, we list some selected  $n^{\text{th}}$  differences, and create conjectures for differences of  $F$ -factors in general.

In Table 8, we list the differences with  $a = b = 1$  for  $r = 2$ . In particular, we list 3 first differences, and at each level one less difference, to support the conjecture that in fact the  $r^{\text{th}}$  differences seem to be constant in representation  $r$ . Further values are listed in the repository. The monomial factors also seem to follow the same pattern within a fixed  $n$  as general differences.

| n | c | r | difference                                                                                                                                                      |
|---|---|---|-----------------------------------------------------------------------------------------------------------------------------------------------------------------|
| 0 | 1 | 2 | $\frac{1}{q^4}$                                                                                                                                                 |
| 0 | 3 | 2 | $\frac{1}{q^4}(A^4q^4 + A^2q^2 + A^2 + 1)$                                                                                                                      |
| 0 | 5 | 2 | $\frac{1}{q^4}(A^8q^8 + A^6q^6 + A^6q^4 + A^4q^4 + A^4q^2 + A^4 + A^2q^2 + A^2 + 1)$                                                                            |
| 0 | 7 | 2 | $\frac{1}{q^4}(A^{12}q^{12} + A^{10}q^{10} + A^{10}q^8 + A^8q^8 + A^8q^6 + A^8q^4 + A^6q^6 + A^6q^4 + A^6q^2 + A^6 + A^4q^4 + A^4q^2 + A^4 + A^2q^2 + A^2 + 1)$ |
| 1 | 1 | 2 | $\frac{A^2}{q^4}(A^2q^4 + q^2 + 1)$                                                                                                                             |
| 1 | 3 | 2 | $\frac{A^4}{q^4}(A^4q^8 + A^2q^6 + A^2q^4 + q^2 + 1)$                                                                                                           |
| 1 | 5 | 2 | $\frac{A^6}{q^4}(A^6q^{12} + A^4q^{10} + A^4q^8 + A^2q^6 + A^2q^4 + q^2 + 1)$                                                                                   |
| 2 | 1 | 2 | $A^4q^2(A^2q^2 + 1)$                                                                                                                                            |
| 2 | 3 | 2 | $A^8q^6(A^2q^2 + 1)$                                                                                                                                            |

Table 8:  $n^{\text{th}}$  differences of  $F$ -factors
